# Supplementary material for: PU-GCN: Point Cloud Upsampling using Graph Convolutional Networks
Source: arXiv:1912.03264 source file (2021-03-29)
Supplement: Supplementary file 1 [file supplement.tex]

% todo:
% R1) Low resolution (res.) experiment. The CD↓ values on PU-GAN dataset: 256 input points, PU-Net (2.93),
% 3PU (2.29), PU-GAN (2.07), PU-GCN (2.01); 512 input
% points, PU-Net (1.62), 3PU (1.18), PU-GAN (1.14), PUGCN (1.01). The complete quantitative results of 256, 512,
% 1024 and 2048 input points on PU1K and PU-GAN dataset
% along with the qualitative examples will be added to the final Supp

% R1&R4) Surface reconstructions. We showed one example of mesh reconstructions for the single object in Supp.
% Fig. 5, where PU-GCN generates a more faithful result than
% other methods. We replicated the mesh reconstructions with
% all the single object qualitative examples, obtaining similar
% results (we will include them in the final version of Supp.).

% R1) Ablation study w.r.t. noise. We decided to compare
% only against PU-GAN, since it consistently outperformed
% PU-Net and 3PU in synthetic as well as real noisy datasets
% (KITTI). We will follow the reviewer’s suggestions and add
% full comparisons with other methods in the Supp

% R4) Large upsampling factor. We apply the pretrained
% model with ×4 upsampling twice to reach ×16 upsampling
% on PU-GAN dataset (with 2048 input points). The CD↓
% values are: PU-Net (0.547), 3PU (0.189), PU-GAN (0.218),
% PU-GCN (0.107). Full results will be added to the final
% Supp. For other upsampling factors that are not powers of
% 4, one can always use farthest point sampling to sample the
% desired number of points, or simply retrain the network.

In this supplementary material, we provide additional content to complement the paper.
First, we compare our proposed NodeShuffle with previous upsampling methods in great details.
Then we discuss the discrepancy between the point-to-surface (P2F) metric and the qualitative performance. 
We further provide qualitative results of PU-Net \cite{yu2018pu}, 3PU\cite{Yifan20193pu} and our PU-GCN on our proposed PU1K dataset.
We also show qualitative experimental results on a new real-scanned dataset (ScanObjectNN \cite{uy-scanobjectnn-iccv19}).
In addition, we discuss the failure case of our PU-GCN.
Finally, we visualize our proposed large-scale dataset PU1K in comparison to PU-GAN's dataset.

%------------  Upsampling Modules
\section{Comparison of Upsampling Modules}
\mysection{Comparison of NodeShuffle with multi-branch MLPs and duplicate-based upsampling}
PU-Net \cite{yu2018pu} concatenates the outputs from a multi-branch MLPs to upsample the point features. 
Multi-branch MLPs operate on each point separately using $1 \times 1 $ convolutions, ignoring any neighborhood information (see \figLabel \ref{fig:multi-branch}). 
3PU \cite{Yifan20193pu} and PU-GAN \cite{li2019pugan} merely duplicate the point features and append with additional feature vectors to distinguish the copied features from the original ones. Then sets of MLPs are used to compress the features (see \figLabel \ref{fig:duplicate}). The duplicate-based method also does not consider the point neighborhood information and will generate points close to the original input due to its duplicate nature.
We note that multi-branch MLPs upsampling can be also viewed as one kind of duplicate-based upsampling: it duplicates the point features and uses separate MLPs to process each copy independently. In our paper, to distinguish the upsampling method used in PU-Net and those used in 3PU and PU-GAN, we refer the upsampling module in PU-Net as Multi-branch MLPs. 
In contrast, our proposed NodeShuffle leverages graph convolution networks (GCNs). GCNs enable our NodeShuffle to encode spatial information from point neighborhoods. The spatial information equips NodeShuffle with the ablity to capture local geometry. 
In addition, our NodeShuffle learns new point from the latent space rather than simply duplicates the original points (unlike 3PU \cite{Yifan20193pu} and PU-GAN \cite{li2019pugan}). 

\begin{figure}[htb!]
\captionsetup[subfigure]{labelformat=empty}
\begin{center}
    \begin{subfigure}{\columnwidth}
             \includegraphics[page=1,trim = 0mm 0mm 20mm 0mm, clip, width=1.0\textwidth]{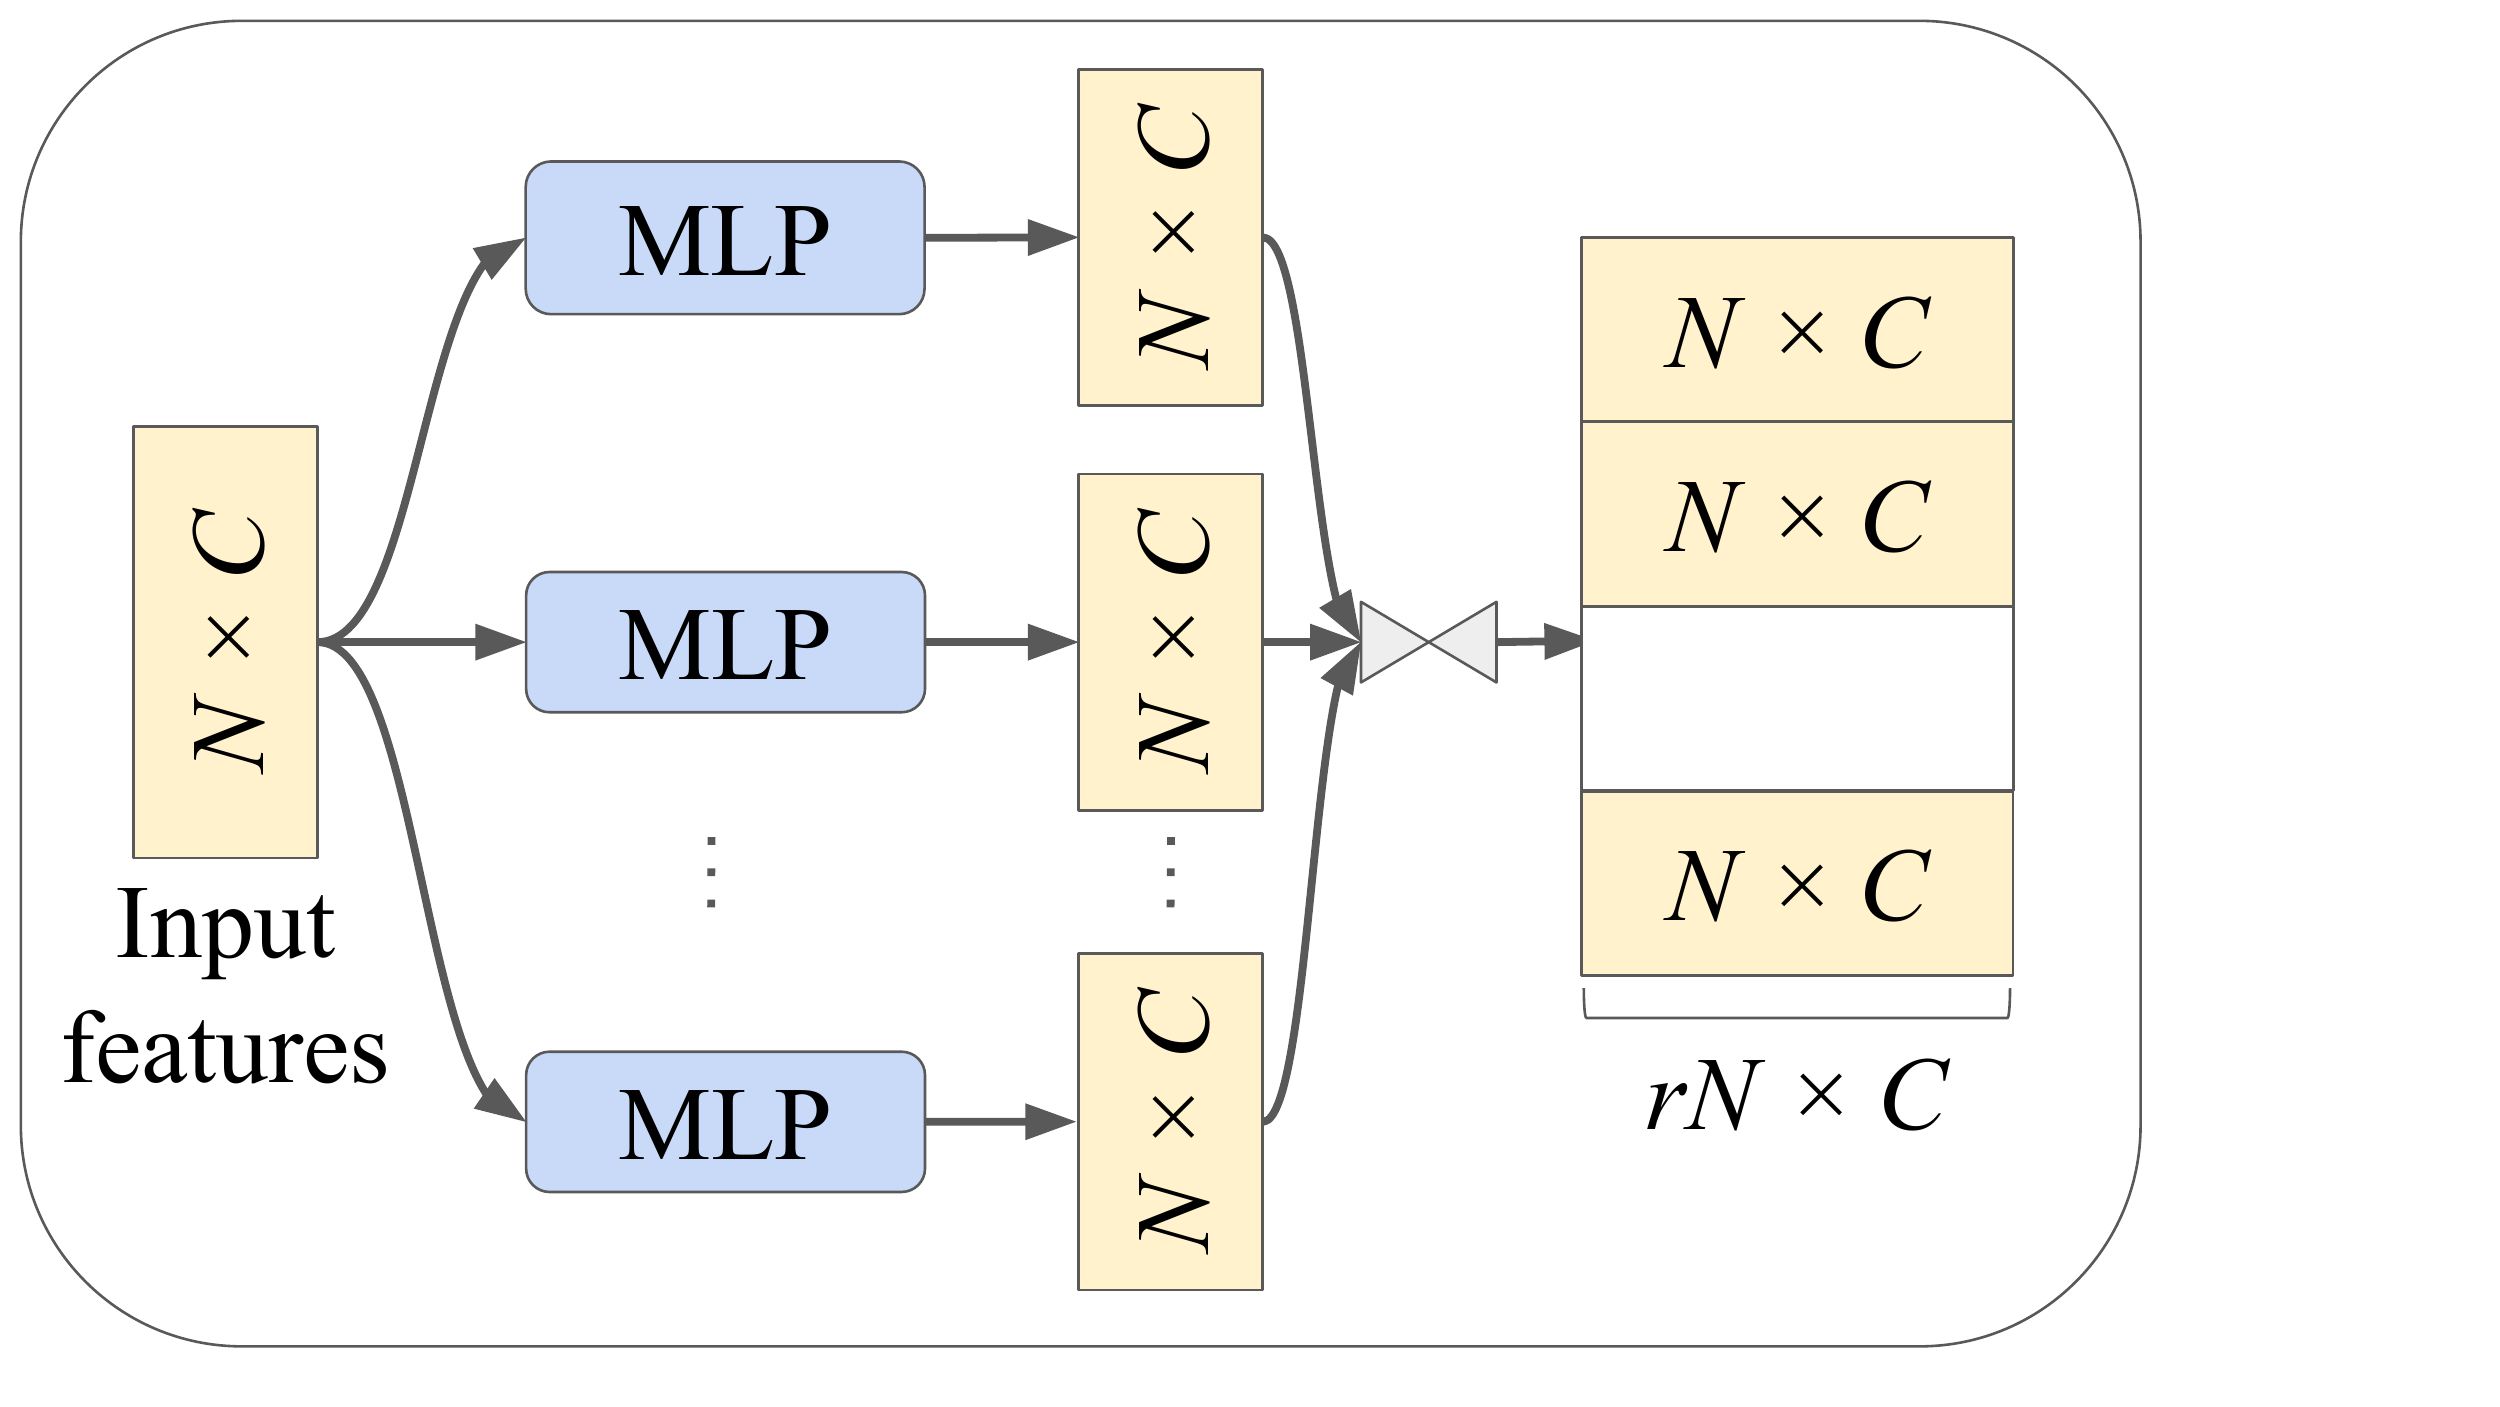}
             \caption{(a) Multi-branch MLPs
             }
             \label{fig:multi-branch}
    \end{subfigure}
    \begin{subfigure}{\columnwidth}
             \includegraphics[page=2,trim = 0mm 30mm 80mm 0mm, clip, width=1.0\textwidth]{figures/pugcn_cvpr21_supp.pdf}
             \caption{(b) Duplicate-based upsampling 
             }
             \label{fig:duplicate}
    \end{subfigure}
\end{center}
\vspace{-10pt}
\caption{\textbf{Previous point upsampling methods.} (a) multi-branch MLPs (used in PU-Net \cite{yu2018pu}): uses MLPs to have point features of different transformations and concatenates those features node-wise; (b) duplicate-based upsampling (used in 3PU \cite{Yifan20193pu} and PU-GAN \cite{li2019pugan}): duplicates the point features and appends with additional feature vectors to distinguish the copied features from the original ones and then uses a set of MLPs to compress the features.
}
\label{fig:previous_upsampling}
\end{figure}

\mysection{Comparison of NodeShuffle with PixelShuffle\cite{Shi2016RealTimeSI}}
PixelShuffle is introduced by Shi \etal \cite{Shi2016RealTimeSI} for the image super-resolution tasks, where the channel expansion and shuffle operation are combined to learn the sub-pixel information in 2D grid data. In our paper, we bring this effective upsampling technique to non-Euclidean data. We adopt GCNs and propose NodeShuffle to learn the sub-point information in the channel expansion part. 

% ------------- Possible Discrepancy 
\section{Discrepancy between P2F and Qualitative Performance}
In the main paper, we show that there exists a discrepancy between the point-to-surface (P2F) metric and qualitative performance. 
\figLabel \ref{fig:p2f} below shows the discrepancy. 
The average of P2F values of our PU-GCN's results are higher than PU-GAN.
However, one can observe that PU-GCN always generates less outliers and higher quality fine-grained details compared to PU-GAN (\eg legs of the bird, between the legs of the camel, and the back of the chair).
P2F is not as reliable as CD and HD for point cloud upsampling. 
We note that only point clouds are considered in the training pipeline. 
The P2F metric uses an unseen input form (mesh) in training may cause the discrepancy in the evaluation for point cloud upsampling.
PU-GCN scores higher P2F than PU-GAN, however PU-GCN is much better in CD and HD as well as the qualitative performance. 

\begin{figure*}[htb!]
\begin{center}
\begin{subfigure}{.3\textwidth}
        \centering
        \includegraphics[page=3,trim = 0mm 0mm 100mm 0mm, clip, width=1.0\columnwidth]{figures/pugcn_cvpr21_supp.pdf}
        \includegraphics[page=6,trim = 0mm 0mm 100mm 0mm, clip, width=1.0\columnwidth]{figures/pugcn_cvpr21_supp.pdf}
        \includegraphics[page=9,trim = 0mm 0mm 100mm 0mm, clip, width=1.0\columnwidth]{figures/pugcn_cvpr21_supp.pdf}
        \caption{Original Mesh}
        
    \end{subfigure}
    \begin{subfigure}{.3\textwidth}
        \centering
        \includegraphics[page=4,trim = 0mm 0mm 100mm 0mm, clip, width=1.0\columnwidth]{figures/pugcn_cvpr21_supp.pdf}
        \includegraphics[page=7,trim = 0mm 0mm 100mm 0mm, clip, width=1.0\columnwidth]{figures/pugcn_cvpr21_supp.pdf}
        \includegraphics[page=10,trim = 0mm 0mm 100mm 0mm, clip, width=1.0\columnwidth]{figures/pugcn_cvpr21_supp.pdf}
        \caption{PU-GAN}
        
    \end{subfigure}
    \begin{subfigure}{.3\textwidth}
        \centering
        \includegraphics[page=5,trim = 0mm 0mm 100mm 0mm, clip, width=1.0\columnwidth]{figures/pugcn_cvpr21_supp.pdf}
        \includegraphics[page=8,trim = 0mm 0mm 100mm 0mm, clip, width=1.0\columnwidth]{figures/pugcn_cvpr21_supp.pdf}
        \includegraphics[page=11,trim = 0mm 0mm 100mm 0mm, clip, width=1.0\columnwidth]{figures/pugcn_cvpr21_supp.pdf}
        \caption{PU-GCN}
    \end{subfigure}
\end{center}
  \caption{\textbf{Visualization of original meshes and upsampling results of PU-GAN and PU-GCN}. 
  PU-GCN generates points with better qualitative performance although PU-GCN scores higher P2F than PU-GAN. 
  }
\label{fig:p2f}
\end{figure*}

\subsection{Qualitative results on PU1K}
\figLabel \ref{fig:qual_results_supp} shows qualitative results of PU-GCN compared to PU-Net\cite{yu2018pu} and 3PU\cite{Yifan20193pu}.
All models are trained on our proposed PU1K dataset.
We do not compare aginst PU-GAN \cite{li2019pugan}, since we were unable to reproduce PU-GAN mainly because of the unstable nature of GAN. 
Our PU-GCN clearly outperforms the previous methods on our proposed challenging PU1K. PU-GCN successfully generates points with much less outliers (refer to the earphone in the first row) and keeps the input shape better with fine-grained details (see the aircraft tail in the second row and the bench in the third row).

\begin{figure*}[htb!]
\begin{center}
%%%%%%%%% 1st example
    \begin{subfigure}{0.19\textwidth}
        \centering
        \includegraphics[page=12,trim = 30mm 20mm 60mm 20mm, width=1.0\textwidth]{figures/pugcn_cvpr21_supp.pdf}
    \end{subfigure}
    \begin{subfigure}{0.19\textwidth}
        \centering
        \includegraphics[page=13,trim = 30mm 20mm 60mm 20mm,
        clip, width=1.0\textwidth]{figures/pugcn_cvpr21_supp.pdf}
    \end{subfigure}
    \begin{subfigure}{0.19\textwidth}
        \centering
        \includegraphics[page=14,trim = 30mm 20mm 60mm 20mm,
        clip, width=1.0\textwidth]{figures/pugcn_cvpr21_supp.pdf}
    \end{subfigure}
    \begin{subfigure}{0.19\textwidth}
        \centering
        \includegraphics[page=15,trim = 30mm 20mm 60mm 20mm, width=1.0\textwidth]{figures/pugcn_cvpr21_supp.pdf}
    \end{subfigure}
    \begin{subfigure}{0.19\textwidth}
        \centering
        \includegraphics[page=16,trim = 30mm 20mm 60mm 20mm, width=1.0\textwidth]{figures/pugcn_cvpr21_supp.pdf}
    \end{subfigure}
    
%%%%%%%%% 2 example
 \begin{subfigure}{0.19\textwidth}
        \centering
        \includegraphics[page=17,trim = 30mm 20mm 60mm 20mm, width=1.0\textwidth]{figures/pugcn_cvpr21_supp.pdf}
    \end{subfigure}
    \begin{subfigure}{0.19\textwidth}
        \centering
        \includegraphics[page=18,trim = 30mm 20mm 60mm 20mm,
        clip, width=1.0\textwidth]{figures/pugcn_cvpr21_supp.pdf}
    \end{subfigure}
    \begin{subfigure}{0.19\textwidth}
        \centering
        \includegraphics[page=19,trim = 30mm 20mm 60mm 20mm,
        clip, width=1.0\textwidth]{figures/pugcn_cvpr21_supp.pdf}
    \end{subfigure}
    \begin{subfigure}{0.19\textwidth}
        \centering
        \includegraphics[page=20,trim = 30mm 20mm 60mm 20mm, width=1.0\textwidth]{figures/pugcn_cvpr21_supp.pdf}
    \end{subfigure}
    \begin{subfigure}{0.19\textwidth}
        \centering
        \includegraphics[page=21,trim = 30mm 20mm 60mm 20mm, width=1.0\textwidth]{figures/pugcn_cvpr21_supp.pdf}
    \end{subfigure}

%%%%%%%%% 3 example
    \begin{subfigure}{0.19\textwidth}
        \centering
        \includegraphics[page=22,trim = 20mm 20mm 60mm 10mm, clip, width=1.0\textwidth]{figures/pugcn_cvpr21_supp.pdf}
        \caption{Input}
    \end{subfigure}
    \begin{subfigure}{0.19\textwidth}
        \centering
        \includegraphics[page=23,trim = 20mm 20mm 60mm 10mm, clip, width=1.0\textwidth]{figures/pugcn_cvpr21_supp.pdf}
        \caption{PU-Net \cite{yu2018pu}}
    \end{subfigure}
    \begin{subfigure}{0.19\textwidth}
        \centering
      \includegraphics[page=24,trim = 20mm 20mm 60mm 10mm, clip, width=1.0\textwidth]{figures/pugcn_cvpr21_supp.pdf}
        \caption{3PU \cite{Yifan20193pu}}
    \end{subfigure}
    \begin{subfigure}{0.19\textwidth}
        \centering
        \includegraphics[page=25,trim = 20mm 20mm 60mm 10mm, clip, width=1.0\textwidth]{figures/pugcn_cvpr21_supp.pdf}
         \caption{PU-GCN (Ours)}
        \label{fig:exp-qual_results-ours}
    \end{subfigure}
    \begin{subfigure}{0.19\textwidth}
        \centering
        \includegraphics[page=26,trim = 20mm 20mm 60mm 10mm, clip, width=1.0\textwidth]{figures/pugcn_cvpr21_supp.pdf}
         \caption{GT}
        \label{fig:exp-qual_results-gt}
    \end{subfigure}
\end{center}
\caption{\textbf{Qualitative upsampling ($\times 4$) results on PU1K.} We show the upsampled point clouds of input (a) when processed by PU-Net\cite{yu2018pu} (b), 3PU\cite{Yifan20193pu} (c) and our proposed PU-GCN (d). The ground truth upsampled point clouds are in (e) for reference. All the inputs are taken from the PU1K test set and have 2048 points. PU-GCN produces the best results overall, while preserving fine-grained local details (refer to close-ups).}
\label{fig:qual_results_supp}
\end{figure*}

%%%%%%%%%%%%%%%%%%%%%%%%%%%%%%%%%%%%%%%%%%%%%%%%%%%%%%%%%%%%%%%%%%%%%%
\section{More real-scanned results}
In the main paper, we provide the results of PU-GCN when used to upsample real-scanned data from the KITTI dataset \cite{Geiger2012CVPR}.
Here, we also experiment with the ScanObjectNN dataset \cite{uy-scanobjectnn-iccv19}. ScanObjectNN contains real-scanned data of various indoor scenes and objects. 
\figLabel \ref{fig:exp-scanobjectnn} shows PU-GCN upsampling results on the original point clouds from the ScanObjectNN dataset. Our PU-GCN trained on PU1K dataset successfully produces high quality upsampled point clouds. 

%------ ScanObjectNN Figures. 
\begin{figure*}[htb!]
\begin{center}
    \begin{subfigure}{\textwidth}
    \centering
             \includegraphics[page=27,trim = 48mm 5mm 50mm 5mm, clip, width=0.23\textwidth]{figures/pugcn_cvpr21_supp.pdf}
             \includegraphics[page=28,trim = 48mm 5mm 50mm 5mm, clip, width=0.23\textwidth]{figures/pugcn_cvpr21_supp.pdf}
             \includegraphics[page=29,trim = 48mm 5mm 50mm 5mm, clip, width=0.23\textwidth]{figures/pugcn_cvpr21_supp.pdf}
             \includegraphics[page=30,trim = 48mm 5mm 50mm 5mm, clip, width=0.23\textwidth]{figures/pugcn_cvpr21_supp.pdf}
    \end{subfigure}
    \begin{subfigure}{\textwidth}
    \centering
             \includegraphics[page=31,trim = 48mm 5mm 50mm 5mm, clip, width=0.23\textwidth]{figures/pugcn_cvpr21_supp.pdf}
             \includegraphics[page=32,trim = 48mm 5mm 50mm 5mm, clip, width=0.23\textwidth]{figures/pugcn_cvpr21_supp.pdf}
             \includegraphics[page=33,trim = 48mm 5mm 50mm 5mm, clip, width=0.23\textwidth]{figures/pugcn_cvpr21_supp.pdf}
             \includegraphics[page=34,trim = 48mm 5mm 50mm 5mm, clip, width=0.23\textwidth]{figures/pugcn_cvpr21_supp.pdf}
    \end{subfigure}
\end{center}
\caption{\textbf{Upsampling real-scanned point clouds from ScanObjectNN dataset \cite{uy-scanobjectnn-iccv19}}. PU-GCN trained on PU1K produces high quality $\times 4$ upsampled point clouds.}
\label{fig:exp-scanobjectnn}
\end{figure*}

%------------
\section{Failure Case}
If the input point cloud has an inherent hole, all existing methods: PU-Net \cite{yu2018pu}, 3PU \cite{Yifan20193pu}, PU-GAN \cite{li2019pugan}, and our PU-GCN, tend to overfill it (see \figLabel \ref{fig:failure_case} below).
This happens because all the methods are designed to generate a (locally) uniformly distributed point cloud rather than distributing the points according to the density of the entire input point cloud. Better upsampling based on the density of the input can be researched to improve the quality.

Nonetheless, our PU-GCN maintains the intrinsic structure better than the state-of-the-art. We believe this is due to our feature extractor Inception DenseGCN being able to extract better multi-scale local information and our GCN-based upsampling moduels being able to capture a better local geometry. 

\begin{figure*}[htb!]
\begin{center}
\begin{subfigure}{0.16\textwidth}
        \centering
        \includegraphics[page=1,trim = 0mm 21mm 0mm 21mm, clip, width=1.0\columnwidth]{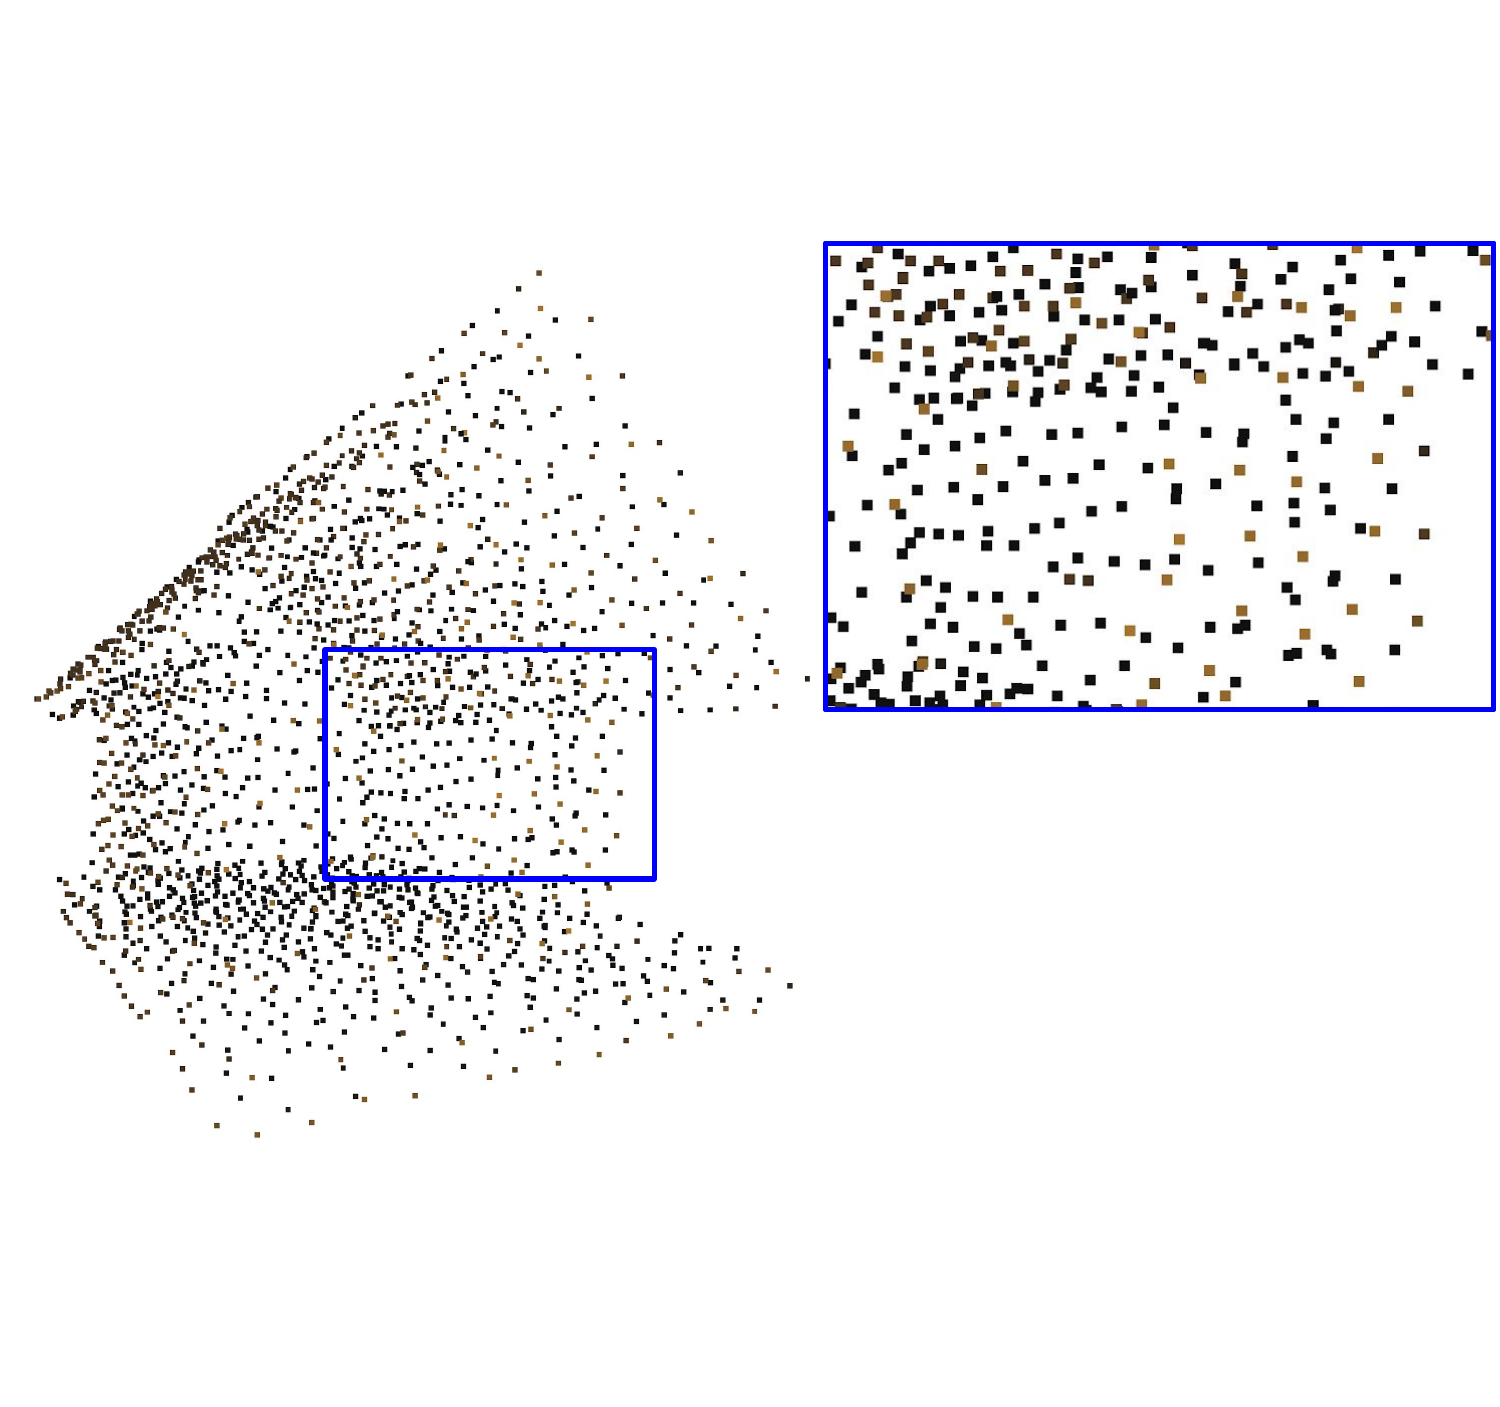}
        \includegraphics[page=2,trim = 0mm 21mm 0mm 21mm, clip, width=1.0\columnwidth]{figures/pugcn_failure_case.pdf}
        \caption{Input}
        
    \end{subfigure}
    \begin{subfigure}{0.16\textwidth}
        \centering
        \includegraphics[page=3,trim = 0mm 21mm 0mm 21mm, clip, width=1.0\columnwidth]{figures/pugcn_failure_case.pdf}
        \includegraphics[page=4,trim = 0mm 21mm 0mm 21mm, clip, width=1.0\columnwidth]{figures/pugcn_failure_case.pdf}
        \caption{PU-Net}
        
    \end{subfigure}
    \begin{subfigure}{0.16\textwidth}
        \centering
        \includegraphics[page=5,trim = 0mm 21mm 0mm 21mm, clip, width=1.0\columnwidth]{figures/pugcn_failure_case.pdf}
        \includegraphics[page=6,trim = 0mm 21mm 0mm 21mm, clip, width=1.0\columnwidth]{figures/pugcn_failure_case.pdf}
        \caption{3PU}
        
    \end{subfigure}
    \begin{subfigure}{0.16\textwidth}
        \centering
        \includegraphics[page=7,trim = 0mm 21mm 0mm 21mm, clip, width=1.0\columnwidth]{figures/pugcn_failure_case.pdf}
        \includegraphics[page=8,trim = 0mm 21mm 0mm 21mm, clip, width=1.0\columnwidth]{figures/pugcn_failure_case.pdf}
        \caption{PU-GAN}
        
    \end{subfigure}
    \begin{subfigure}{0.16\textwidth}
        \centering
        \includegraphics[page=9,trim = 0mm 21mm 0mm 21mm, clip, width=1.0\columnwidth]{figures/pugcn_failure_case.pdf}
        \includegraphics[page=10,trim = 0mm 21mm 0mm 21mm, clip, width=1.0\columnwidth]{figures/pugcn_failure_case.pdf}
        \caption{PU-GCN}
        
    \end{subfigure}
    \begin{subfigure}{0.16\textwidth}
        \centering
        \includegraphics[page=11,trim = 0mm 21mm 0mm 21mm, clip, width=1.0\columnwidth]{figures/pugcn_failure_case.pdf}
        \includegraphics[page=12,trim = 0mm 21mm 0mm 21mm, clip, width=1.0\columnwidth]{figures/pugcn_failure_case.pdf}
        \caption{GT}
    \end{subfigure}
\end{center}
  \caption{\textbf{Failure case} (the birdhouse from our PU1K testing dataset, the upsampling ratio is $\times 4$). All the existing methods, PU-Net \cite{yu2018pu}, 3PU \cite{Yifan20193pu}, PU-GAN \cite{li2019pugan} and our PU-GCN, tend to overfill the inherent holes.}
\label{fig:failure_case}
\end{figure*}

%%%%%%%%%%%%%%%%%%%%%% PU1K
\section{Details of Proposed Dataset PU1K}
We compile \emph{PU1K}, a new large-scale dataset with various levels of shape complexity.
Our PU1K is 8 times bigger than the largest publicly available point upsampling dataset (PU-GAN's dataset \cite{li2019pugan}).
PU1K was compiled from 50 categories ShapeNetCore \cite{shapenet} (compared to only 10 categories in PU-GAN's dataset). We collected 20 models from each category, and resulted in 1,000 models in total (900 in training split and 100 in testing split).
We also added the models from PU-GAN into PU1K and finally obtained 1,147 3D models (1020 in training and 127 in testing). 
Overall, PU1K covers a great semantic range of 3D objects and includes simple, as well as complex shapes. 
\figLabel \ref{fig:training_PU1K_samples} show a sample from each category from our PU1K dataset (without PU-GAN's data). \figLabel \ref{fig:testing_PU1K_samples} show the testing samples from our PU1K dataset (without PU-GAN's data) .
We also show some examples from PU-GAN's dataset in \figLabel \ref{fig:training_pugan_samples} and \figLabel \ref{fig:testing_pugan_samples}. 
One can observe that our PU1K dataset contains models from a larger range of categories and with more shape diversity.

%%%%%%%%%%%%%%%%%%%%%%%%%%%%%%%%%%%%%%%%%%%%
\begin{figure*}[htb!]
\begin{center}
    \includegraphics[page=35,trim = 0mm 0mm 120mm 0mm, clip, width=0.99\textwidth]{figures/pugcn_cvpr21_supp.pdf}
\end{center}
\caption{\textbf{Training samples from PU1K.}}
\label{fig:training_PU1K_samples}
\end{figure*}
 \clearpage
 
\begin{figure*}[htb!]
\begin{center}
    \includegraphics[page=36,trim = 0mm 0mm 160mm 0mm, clip, width=0.9\textwidth]{figures/pugcn_cvpr21_supp.pdf}
\end{center}
  \caption{\textbf{The 100 testing models from PU1K.}}
\label{fig:testing_PU1K_samples}
\end{figure*}

\begin{figure*}[htb!]
\begin{center}
    \includegraphics[page=37,trim = 0mm 0mm 0mm 0mm, clip, width=0.99\textwidth]{figures/pugcn_cvpr21_supp.pdf}
\end{center}
\caption{\textbf{Training samples from PU-GAN's Dataset.}}
\label{fig:training_pugan_samples}
\end{figure*}

\begin{figure*}[htb!]
\begin{center}
    \includegraphics[page=38,trim = 0mm 0mm 0mm 0mm, clip, width=0.99\textwidth]{figures/pugcn_cvpr21_supp.pdf}
\end{center}
\vspace{-10pt}
  \caption{\textbf{Testing samples from PU-GAN's Dataset.}}
\label{fig:testing_pugan_samples}
\end{figure*}
