# Supplementary material for: PU-GCN: Point Cloud Upsampling using Graph Convolutional Networks
Source: arXiv:1912.03264 source file (2021-03-29)

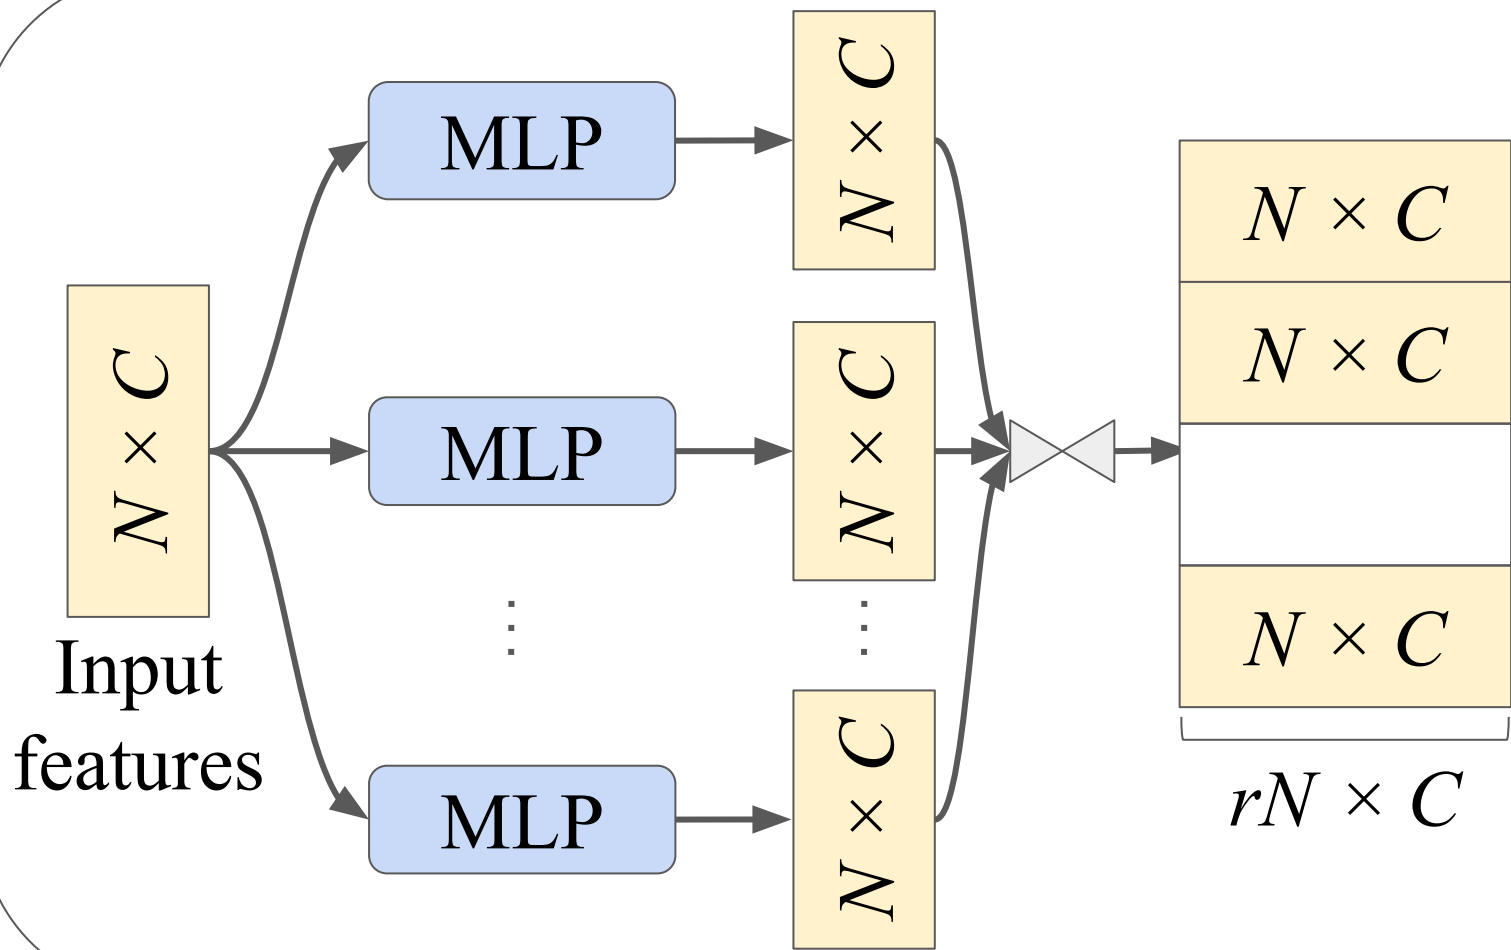

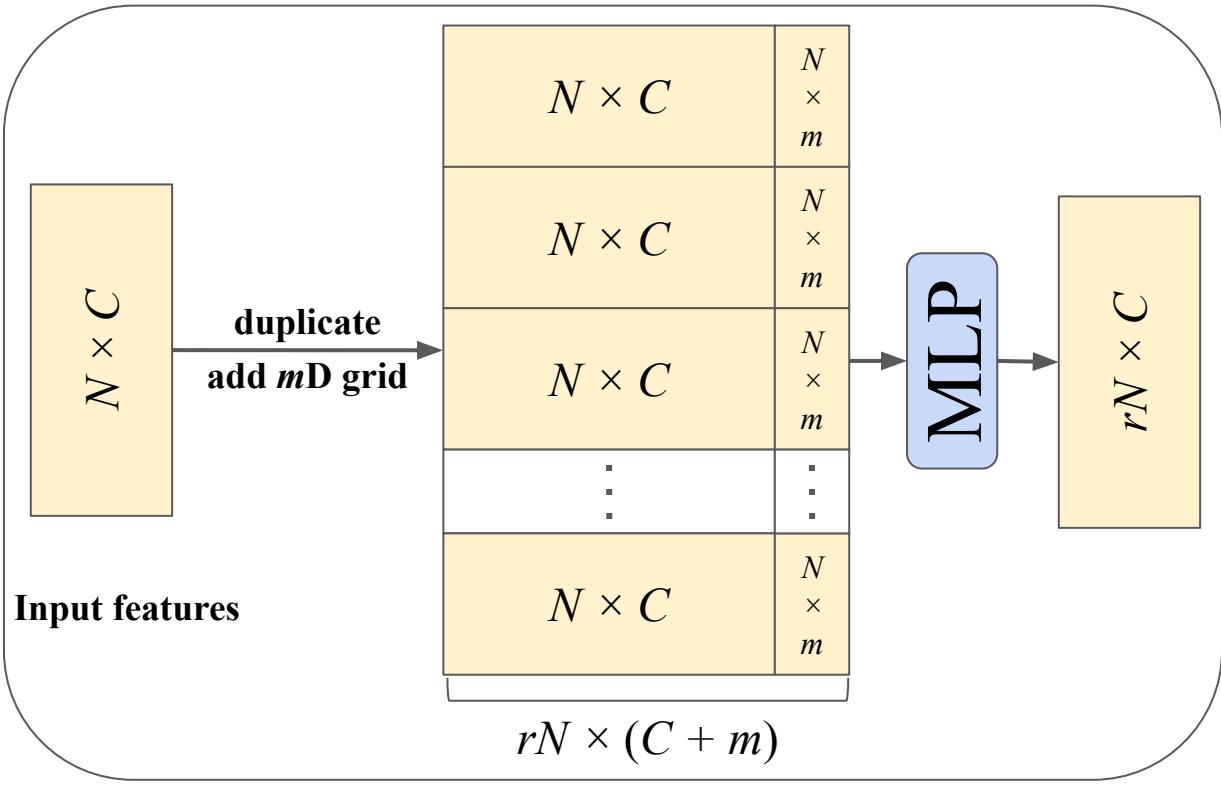

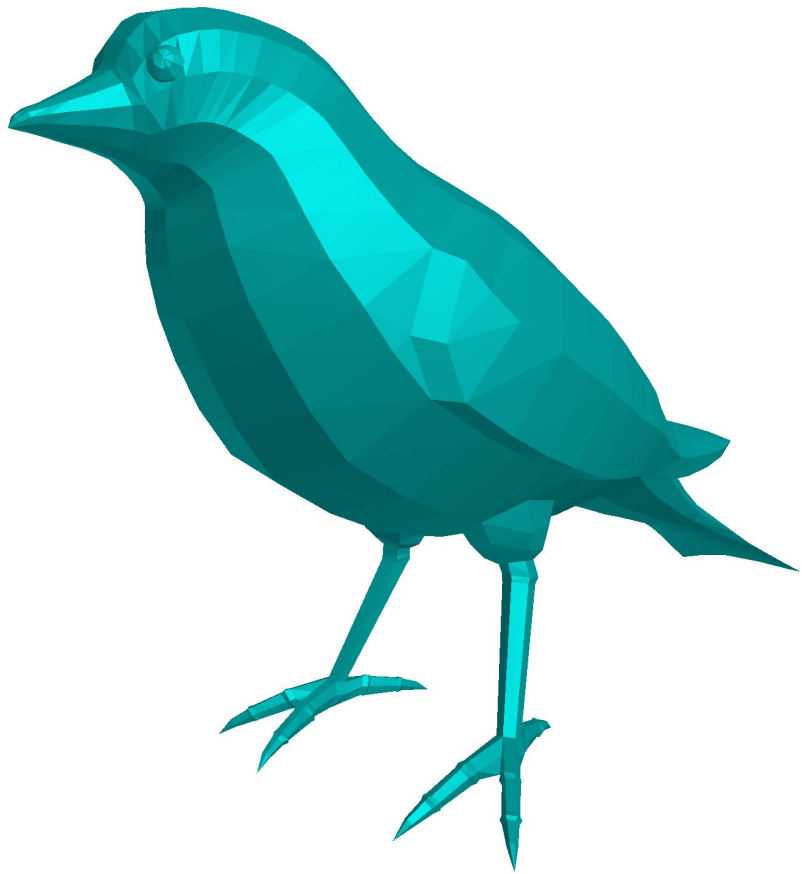

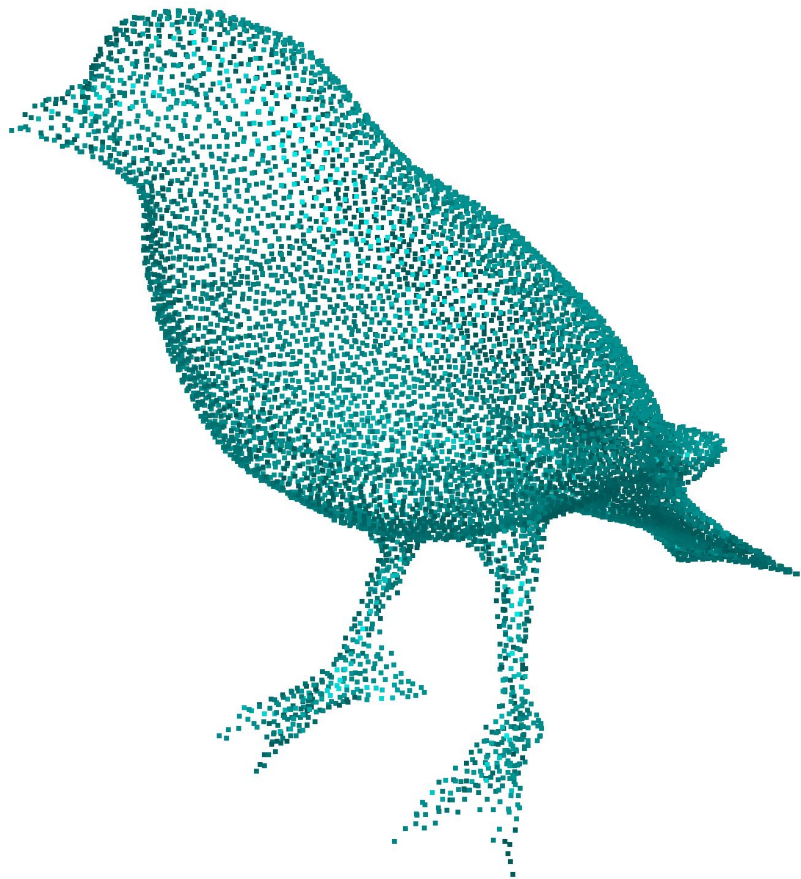

Average P2F =  $1.168 \times 10^{-3}$   
Standard Deviation =  $2.262 \times 10^{-3}$



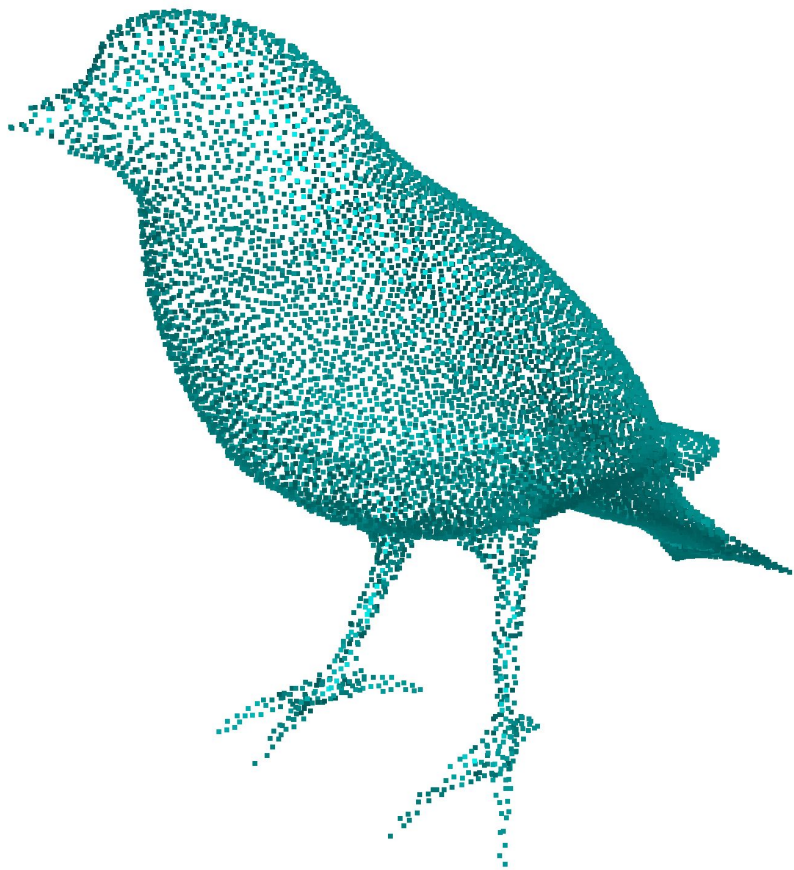

Average P2F =  $1.757 \times 10^{-3}$   
Standard Deviation =  $1.452 \times 10^{-3}$

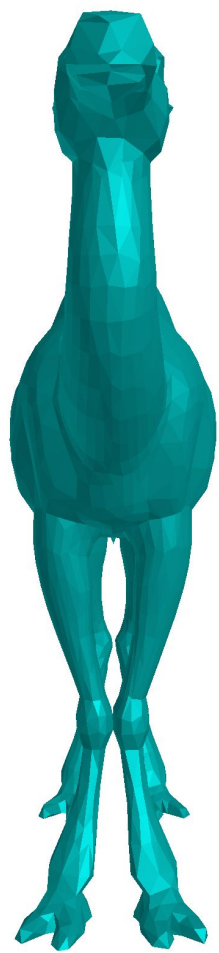

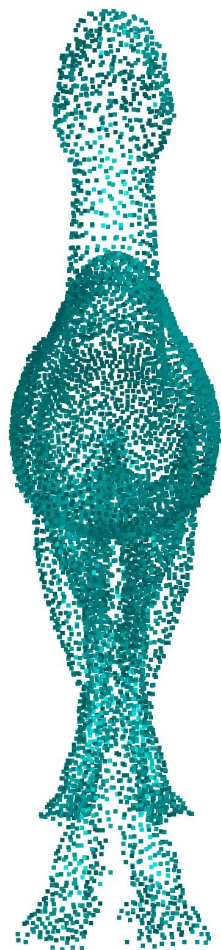

Average P2F =  $1.885 \times 10^{-3}$   
Standard Deviation =  $3.324 \times 10^{-3}$

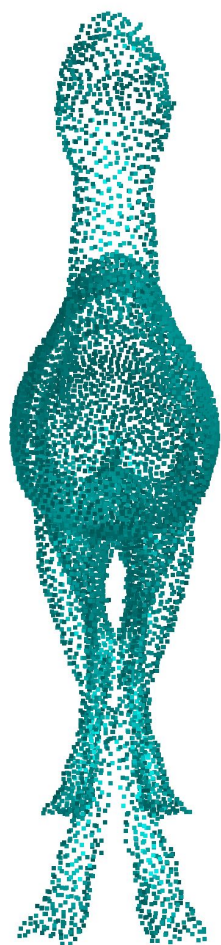

Average P2F =  $2.342 \times 10^{-3}$   
Standard Deviation =  $1.989 \times 10^{-3}$

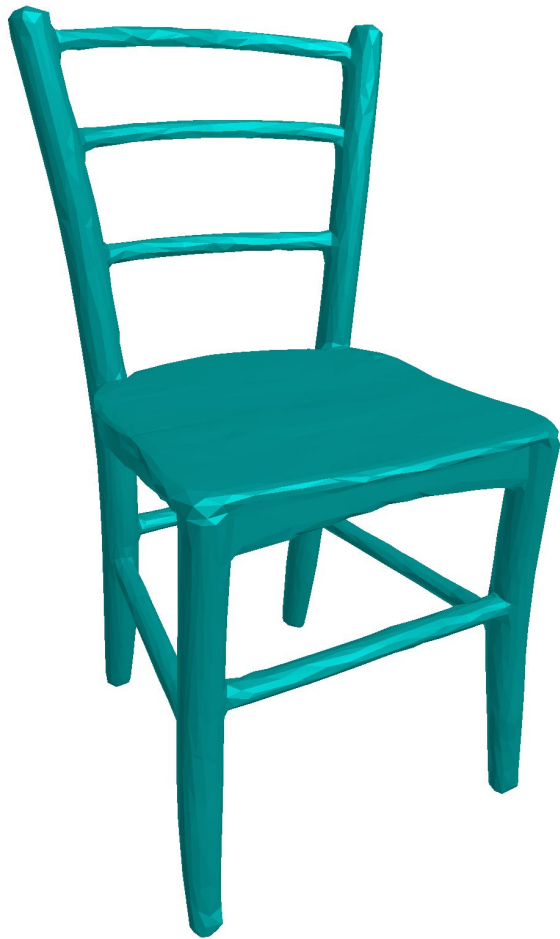

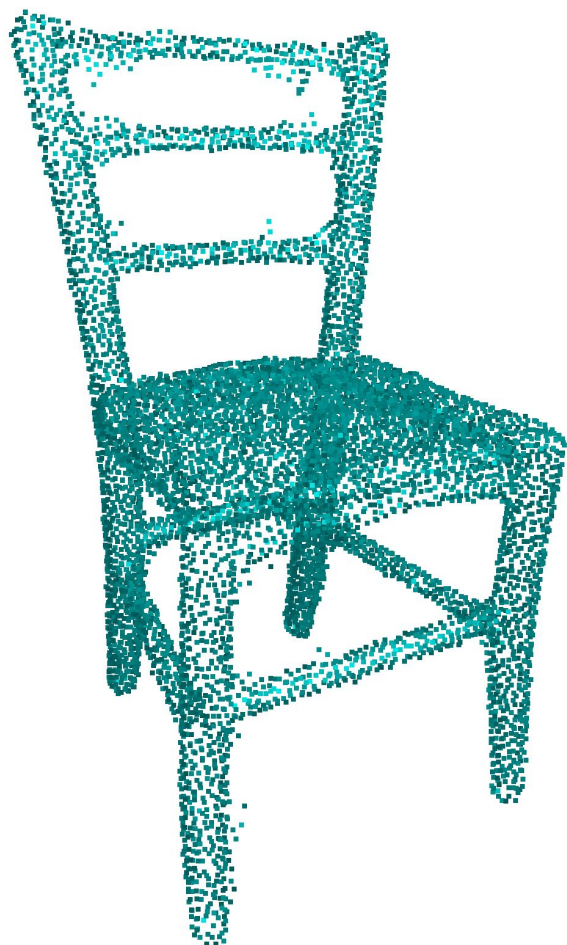

Average P2F =  $2.566 \times 10^{-3}$   
Standard Deviation =  $3.988 \times 10^{-3}$

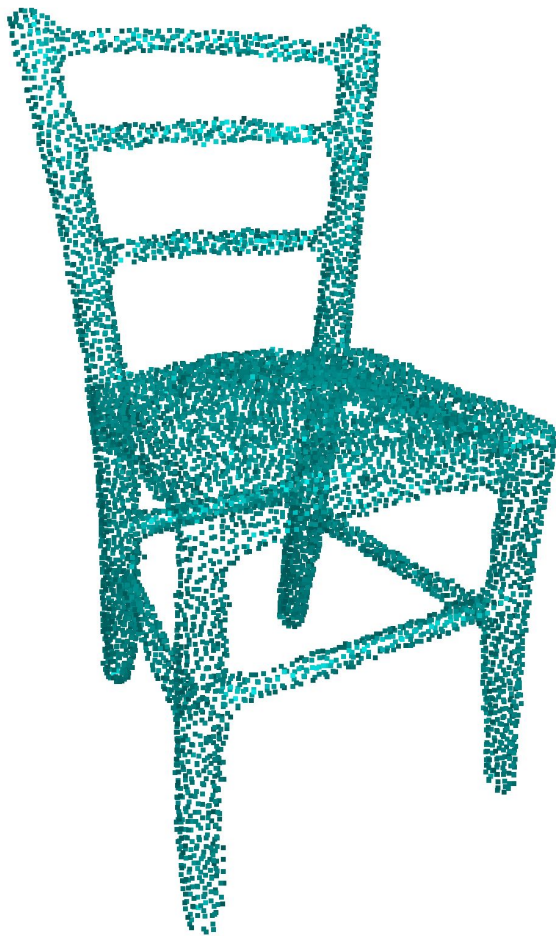

Average P2F =  $3.103 \times 10^{-3}$   
Standard Deviation =  $2.586 \times 10^{-3}$

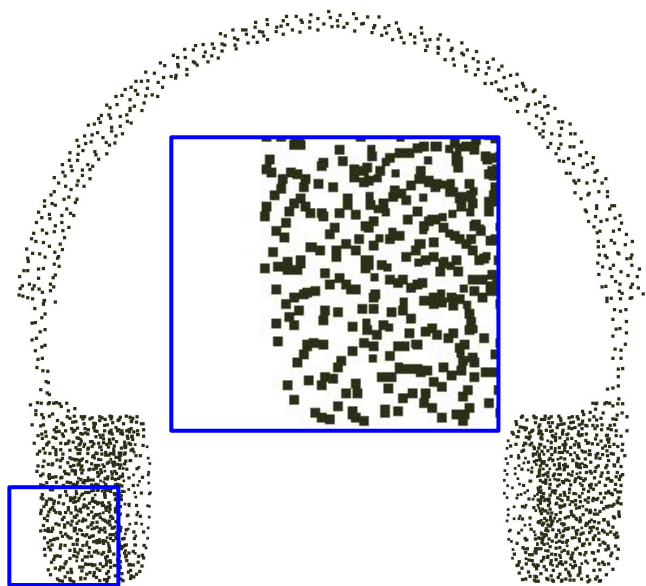



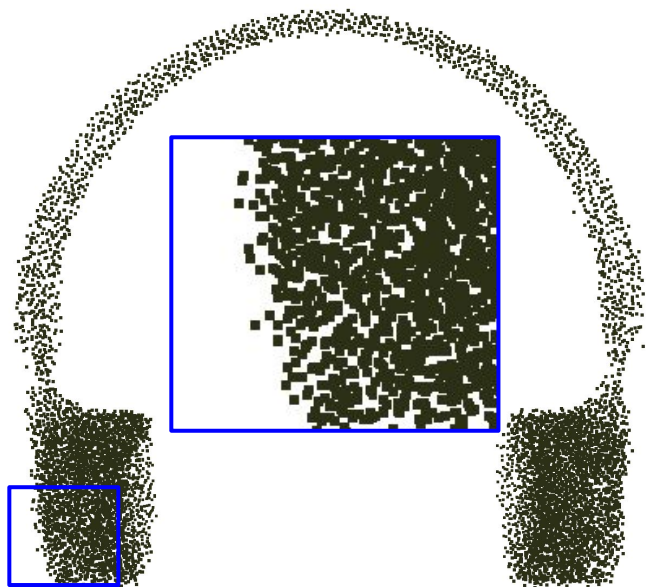

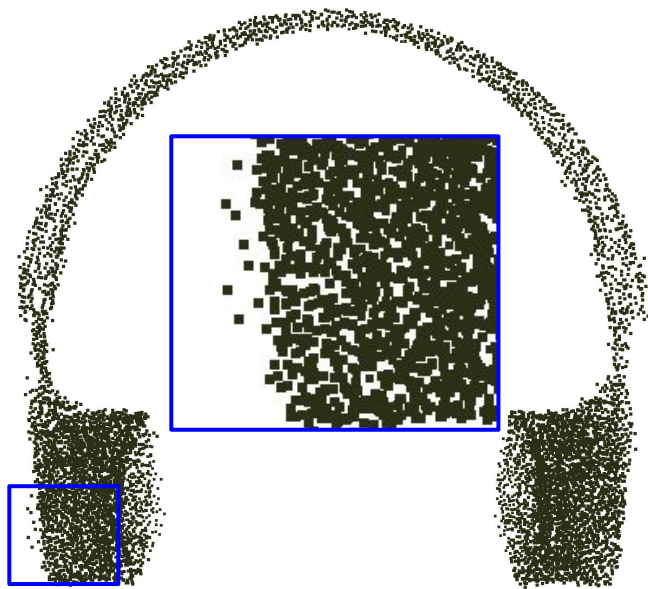

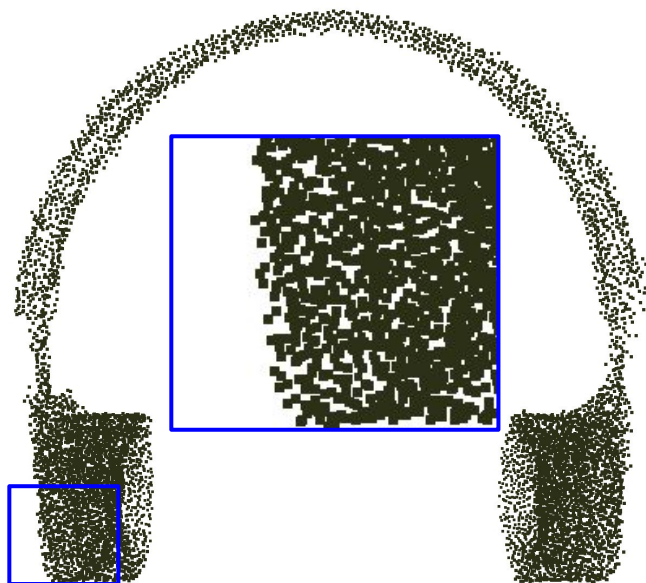

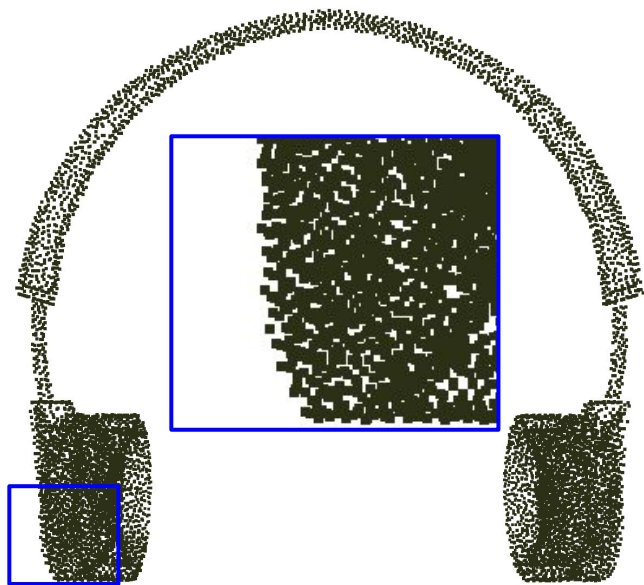

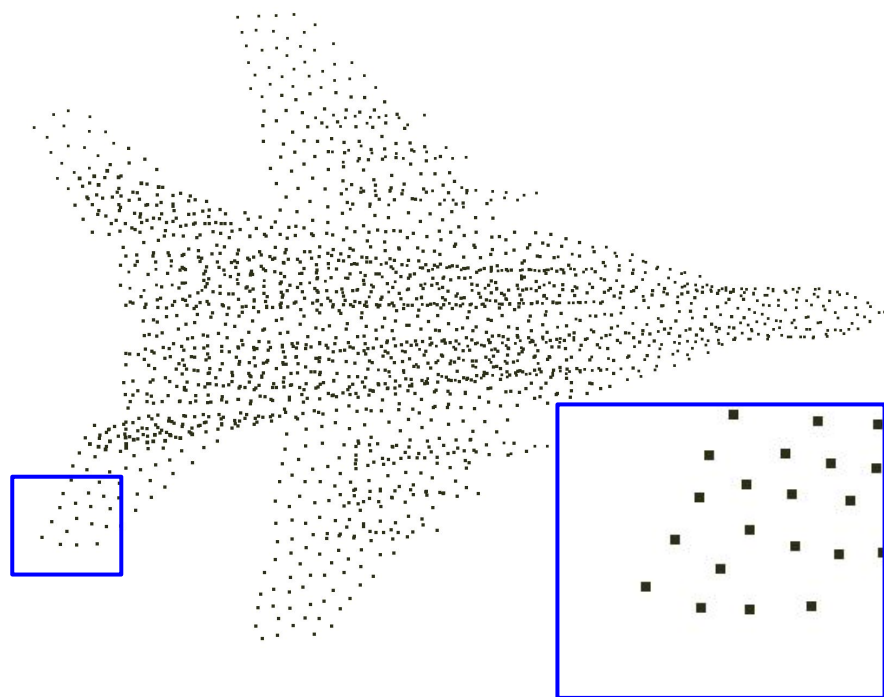

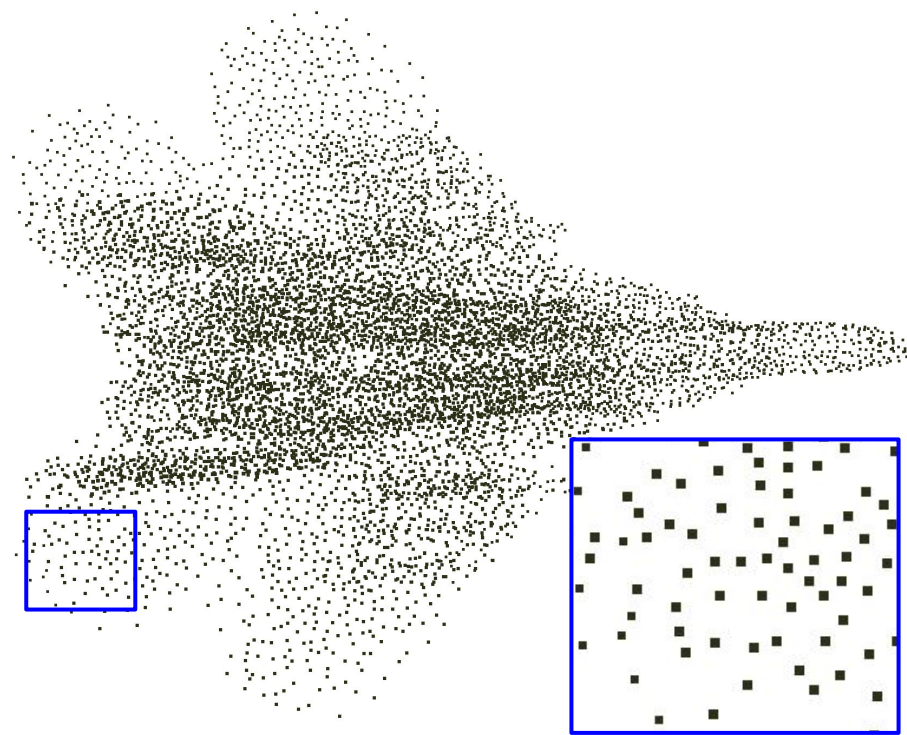

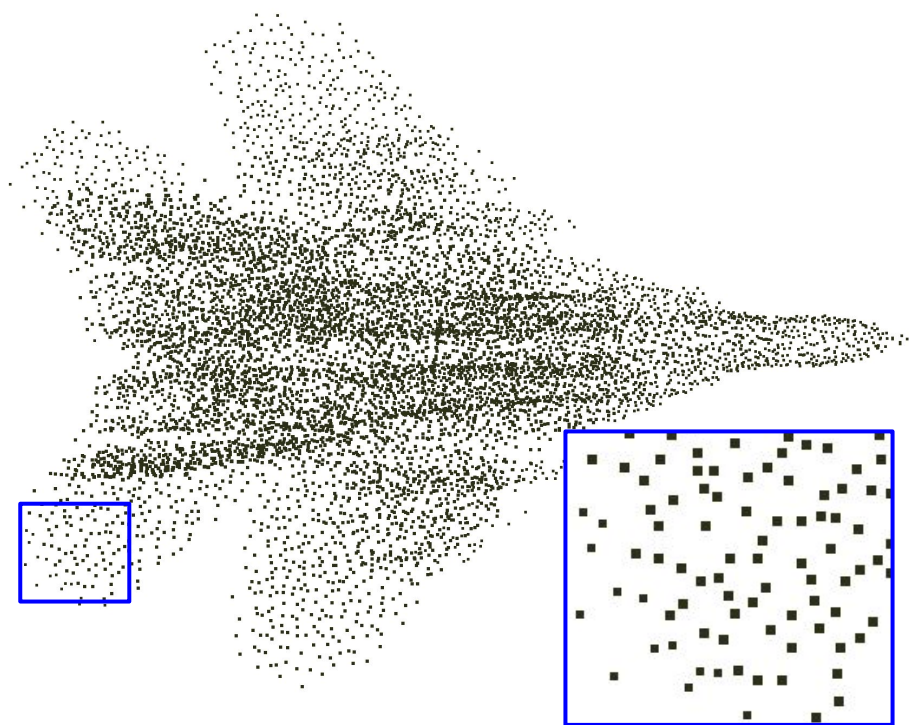

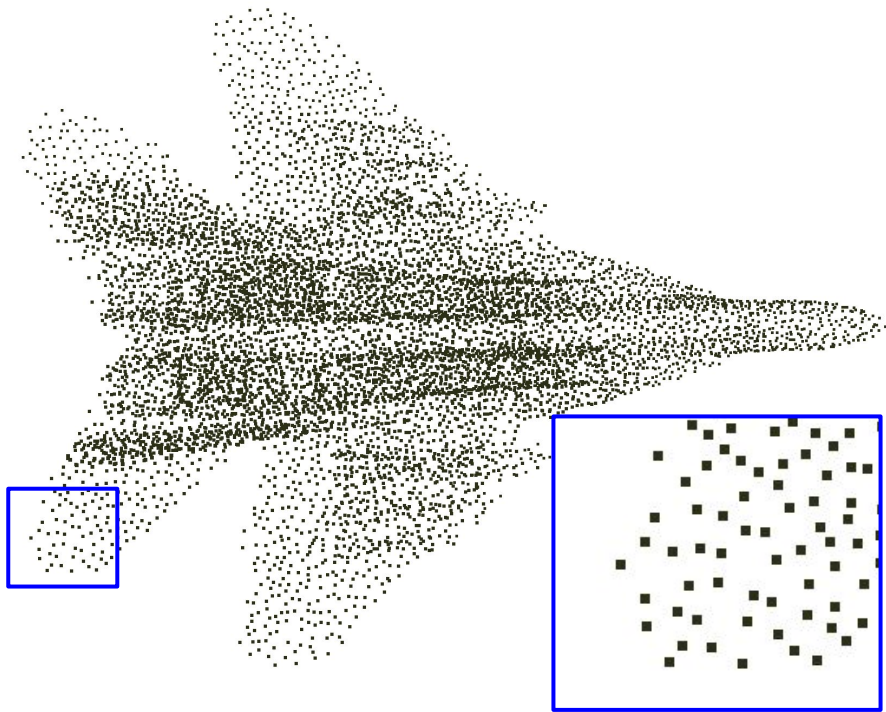



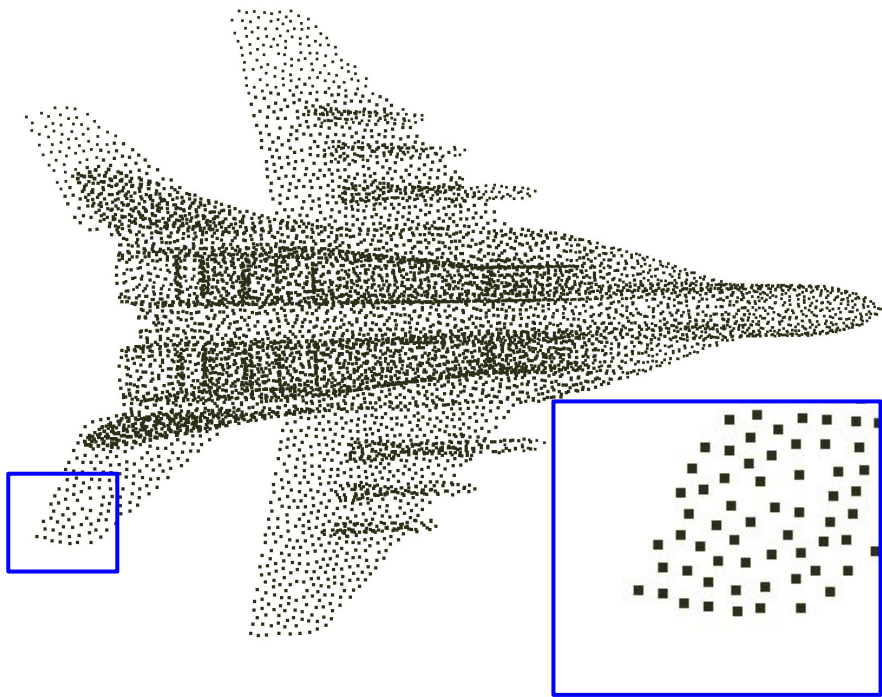

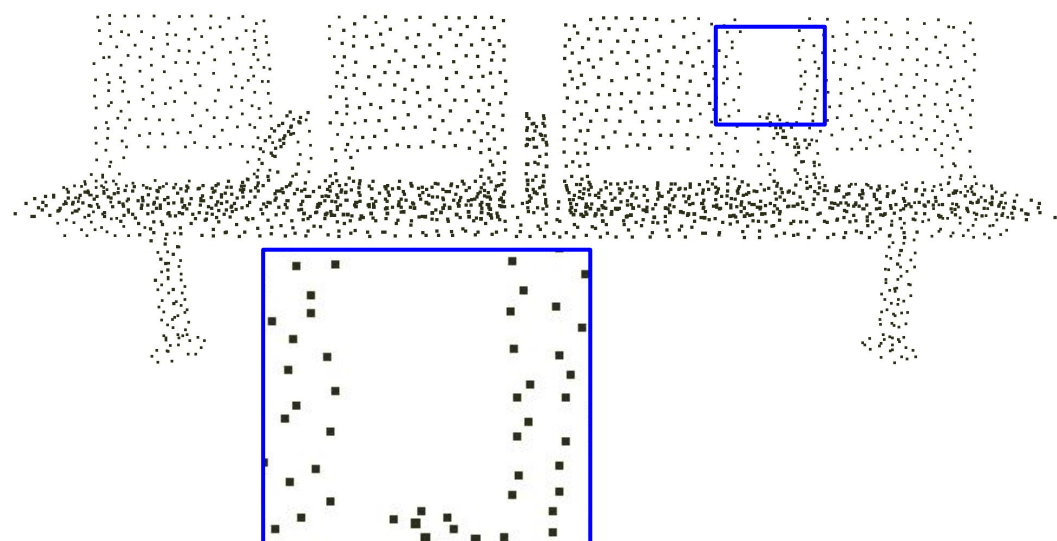

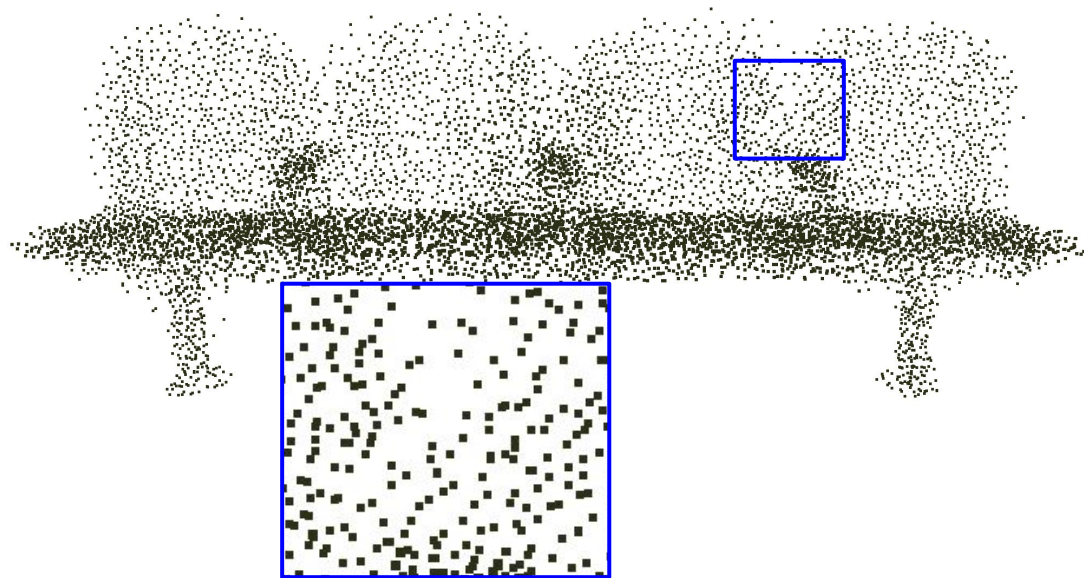

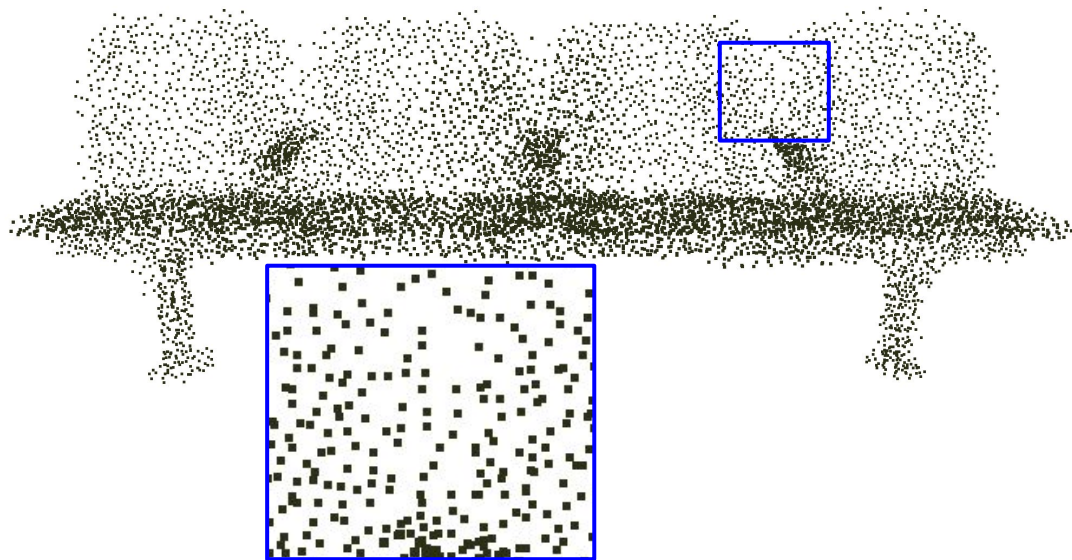

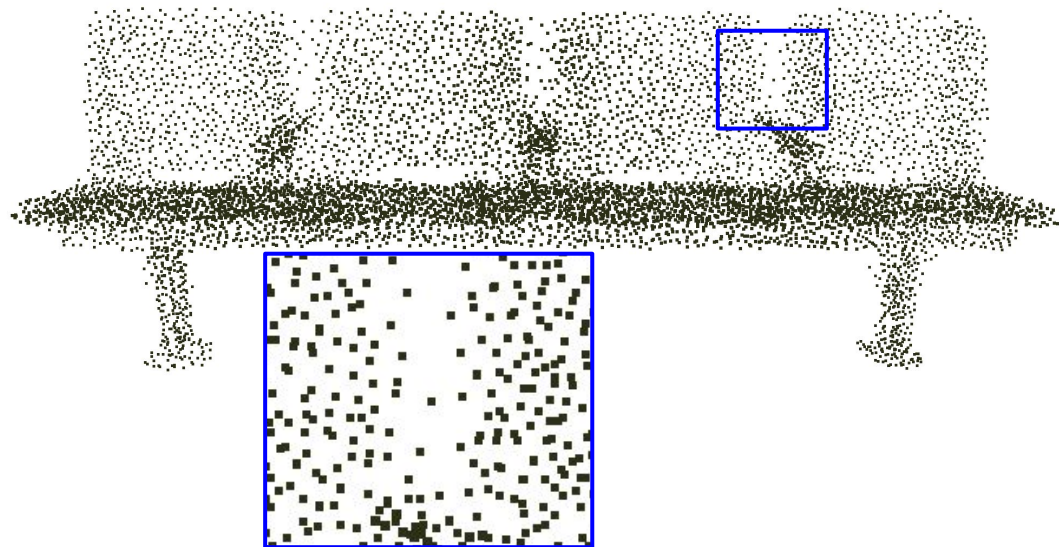

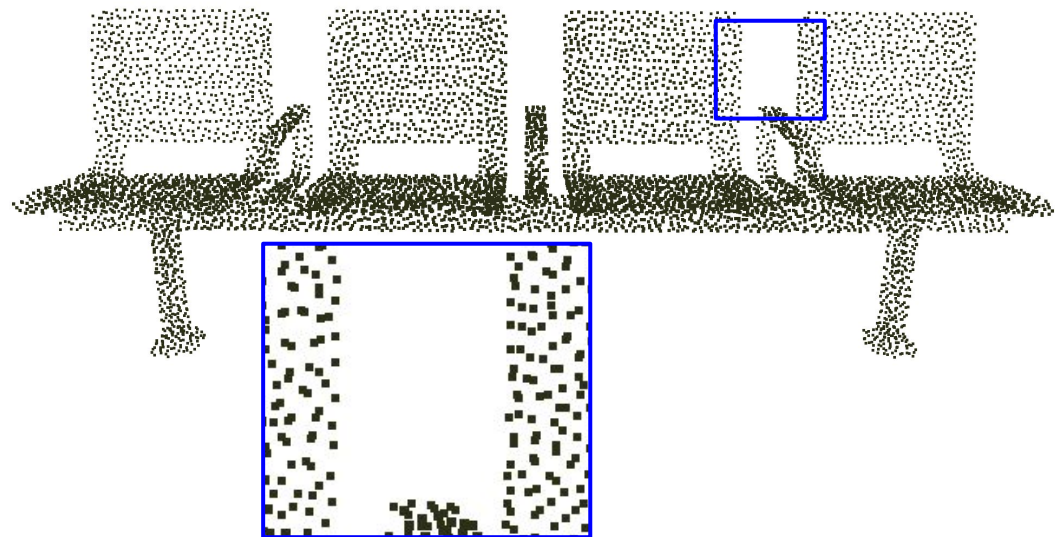

# Input

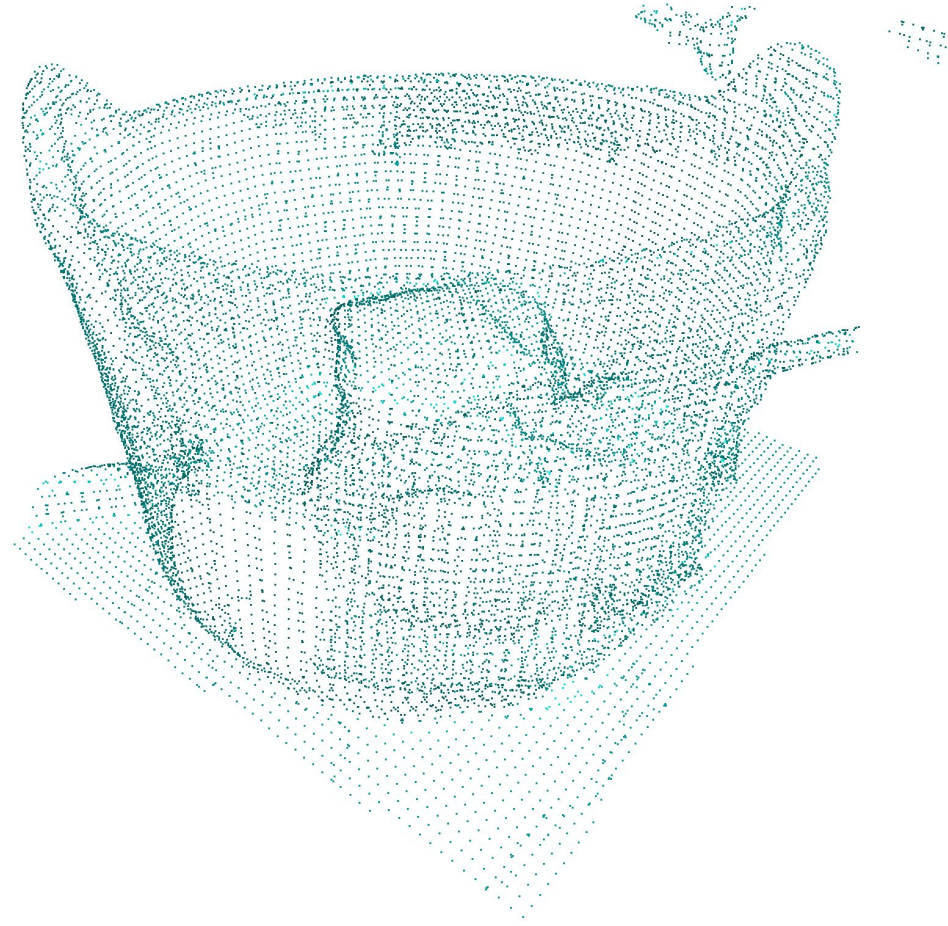



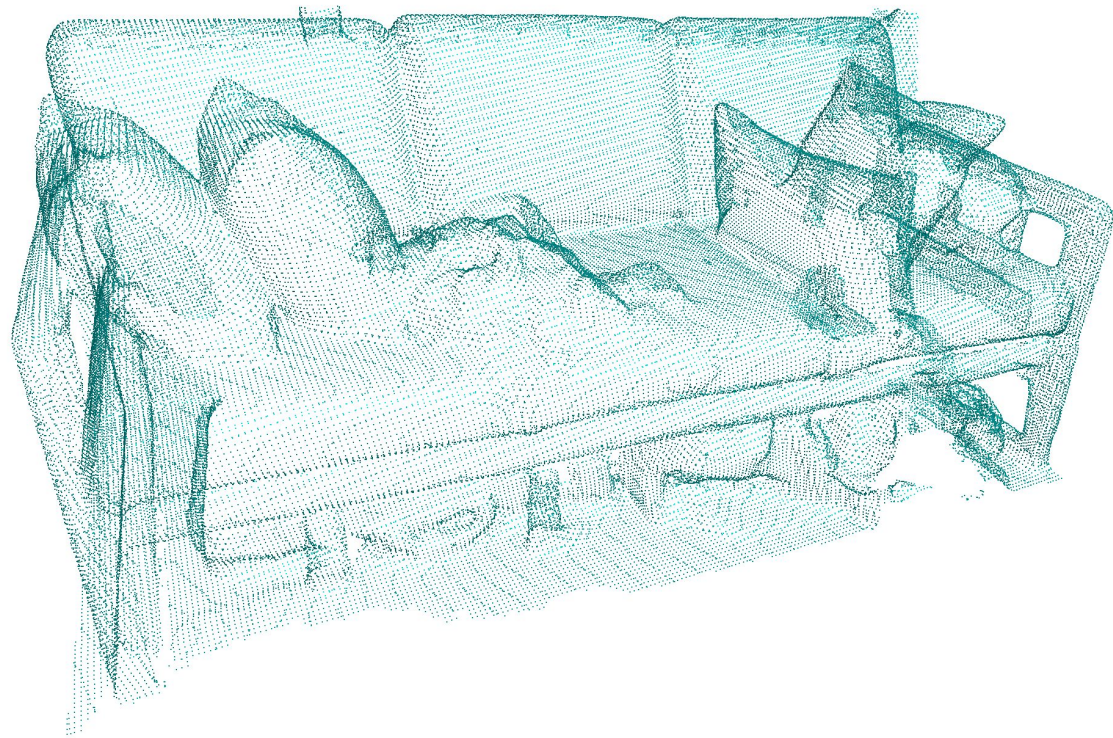



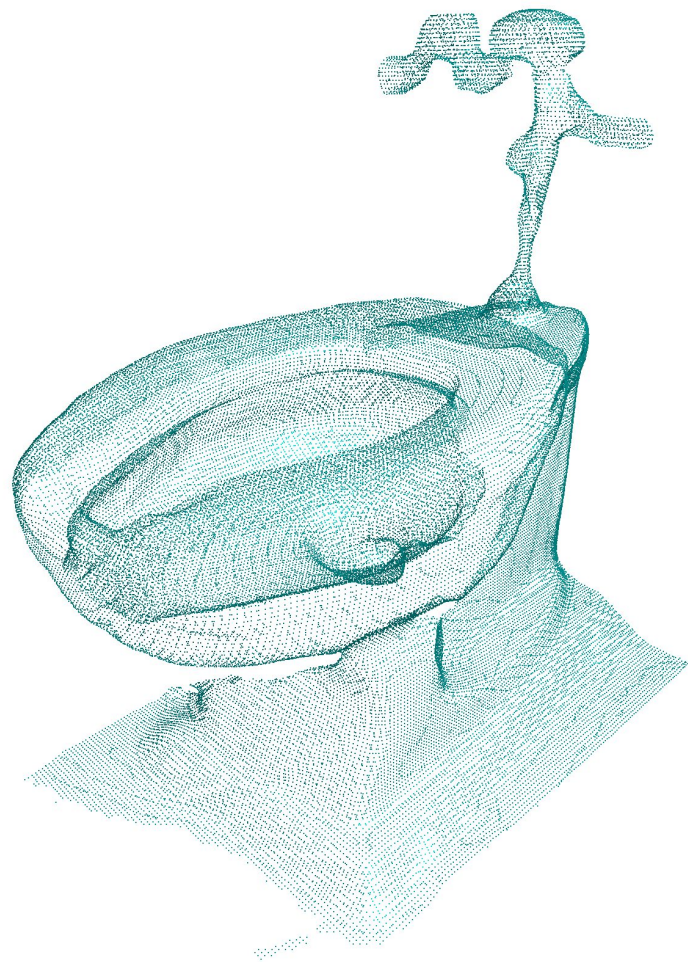

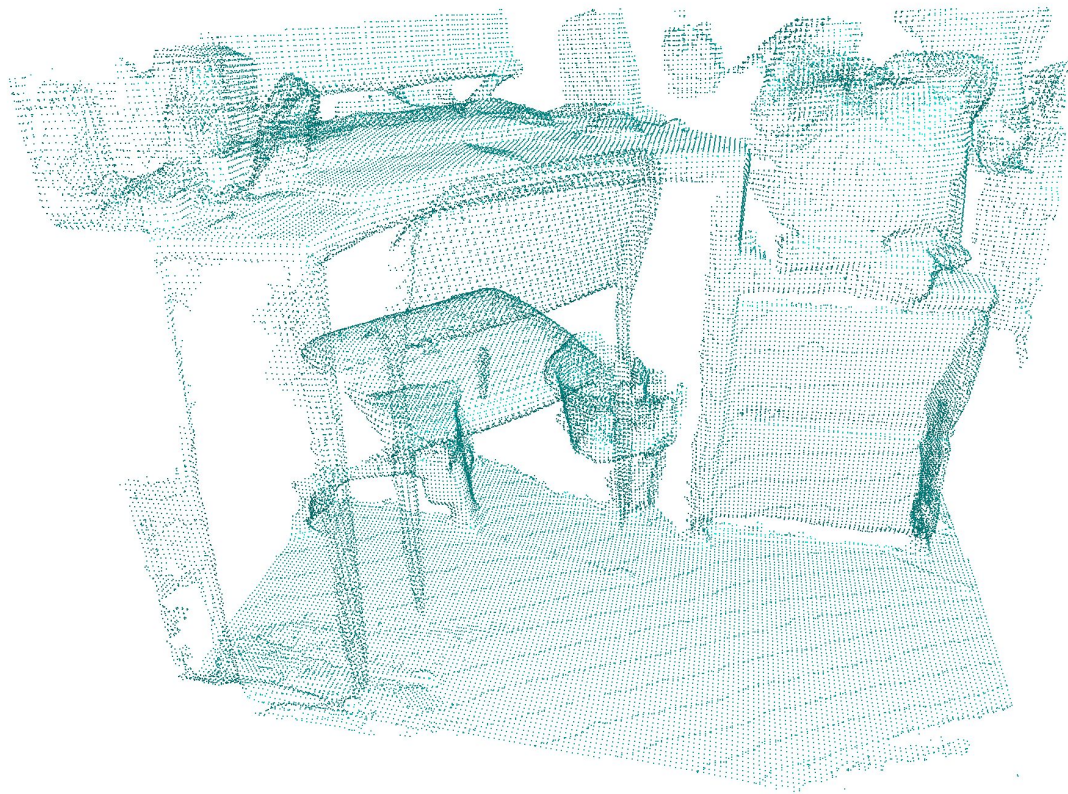

# PU-GCN

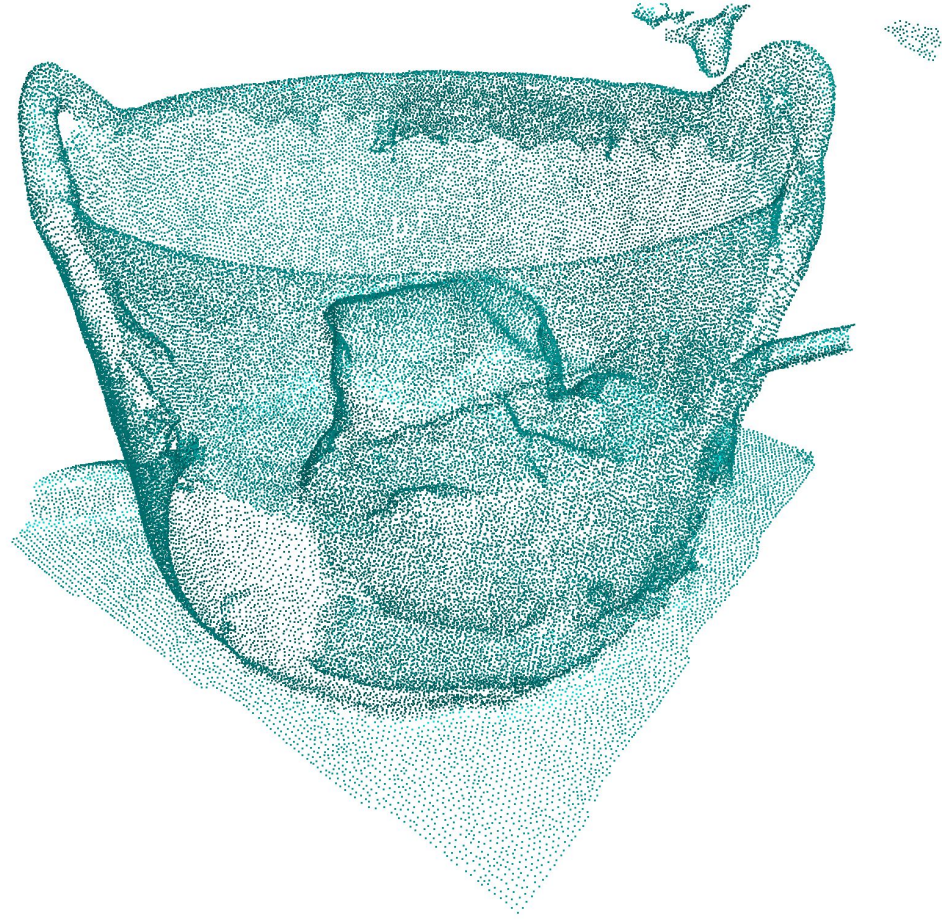



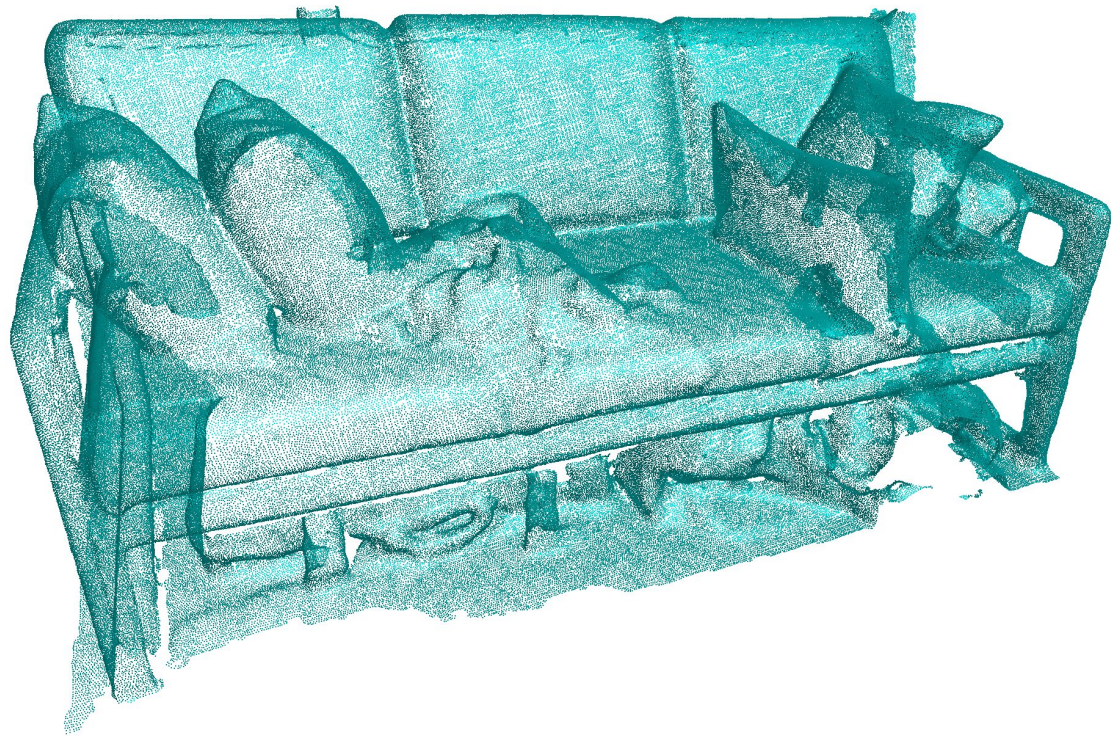

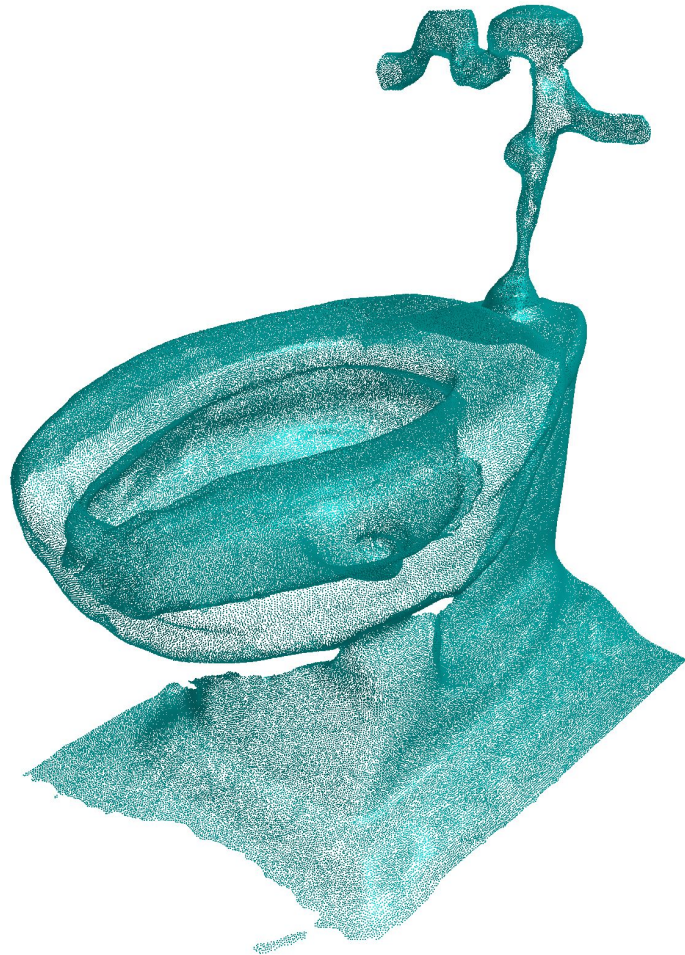



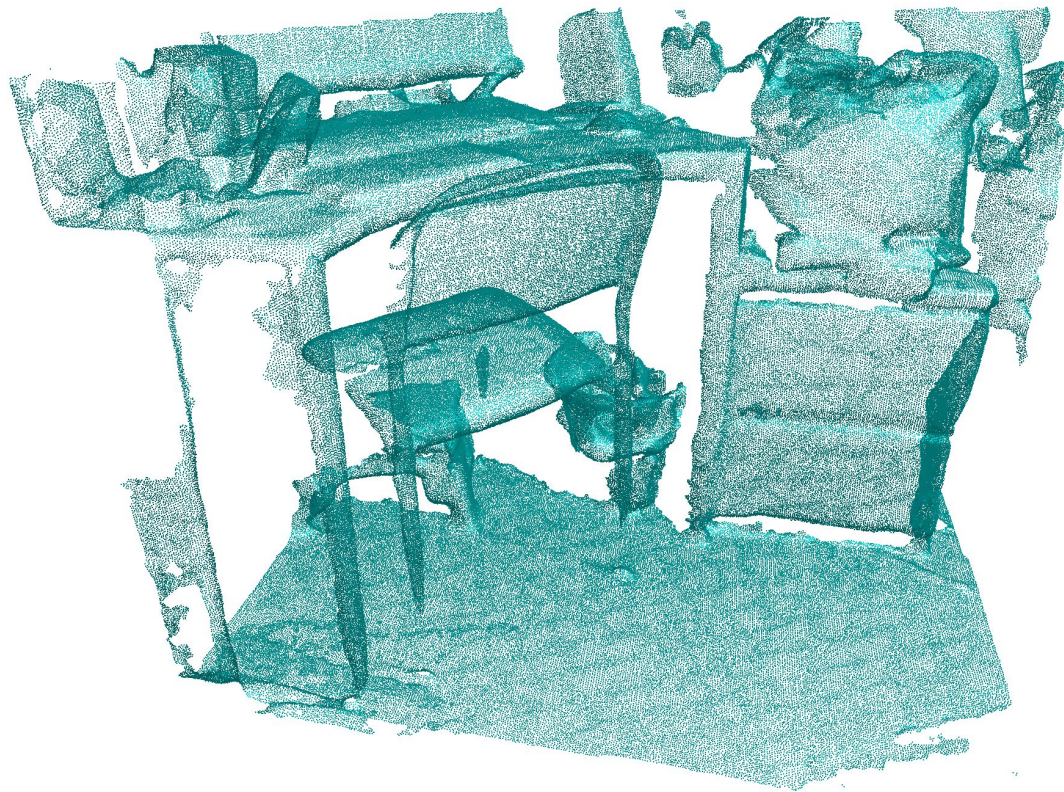

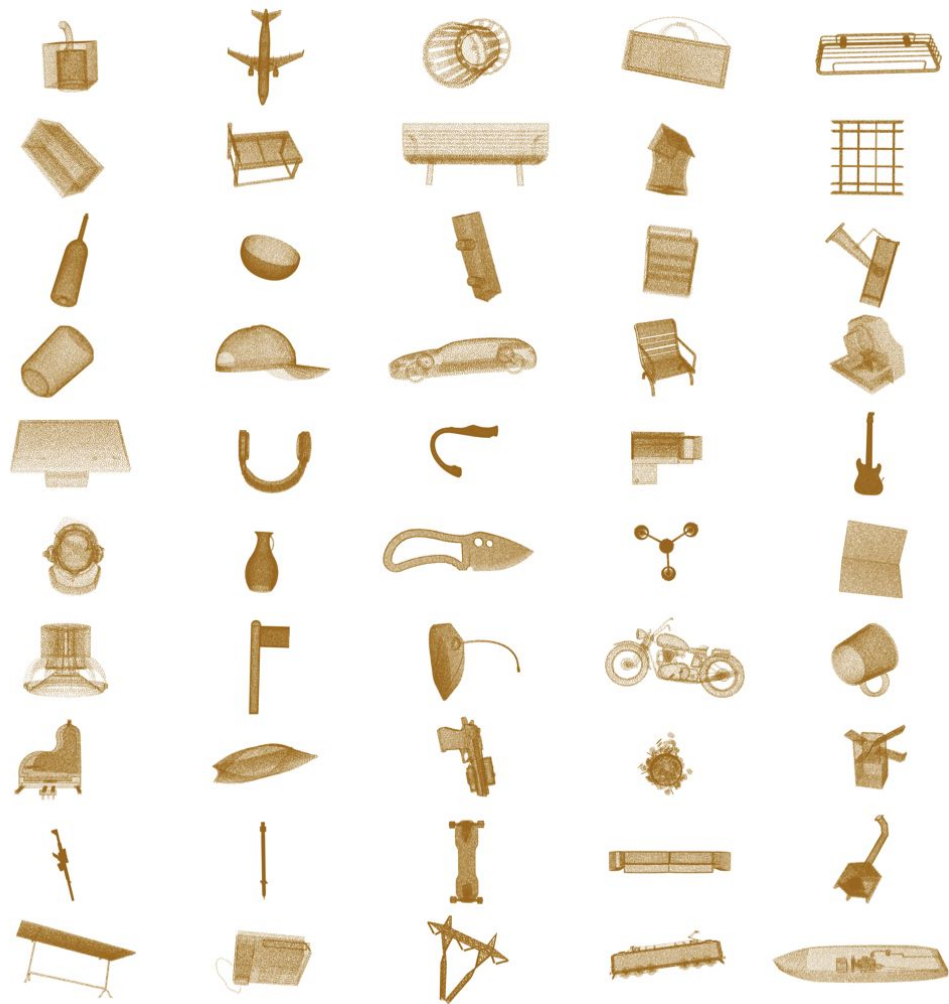

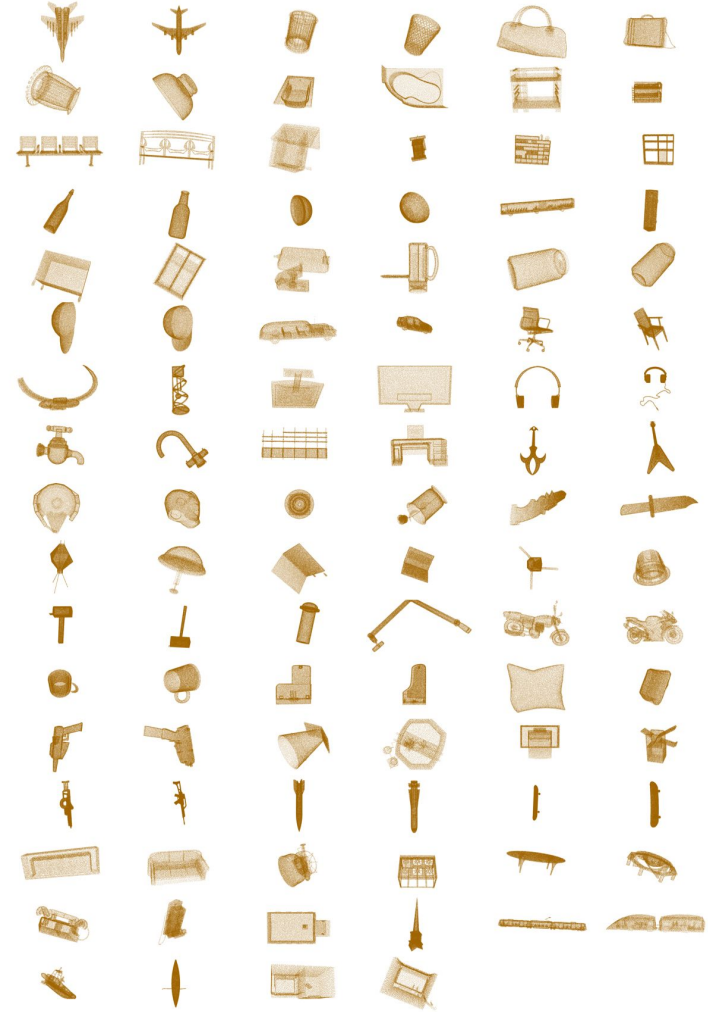



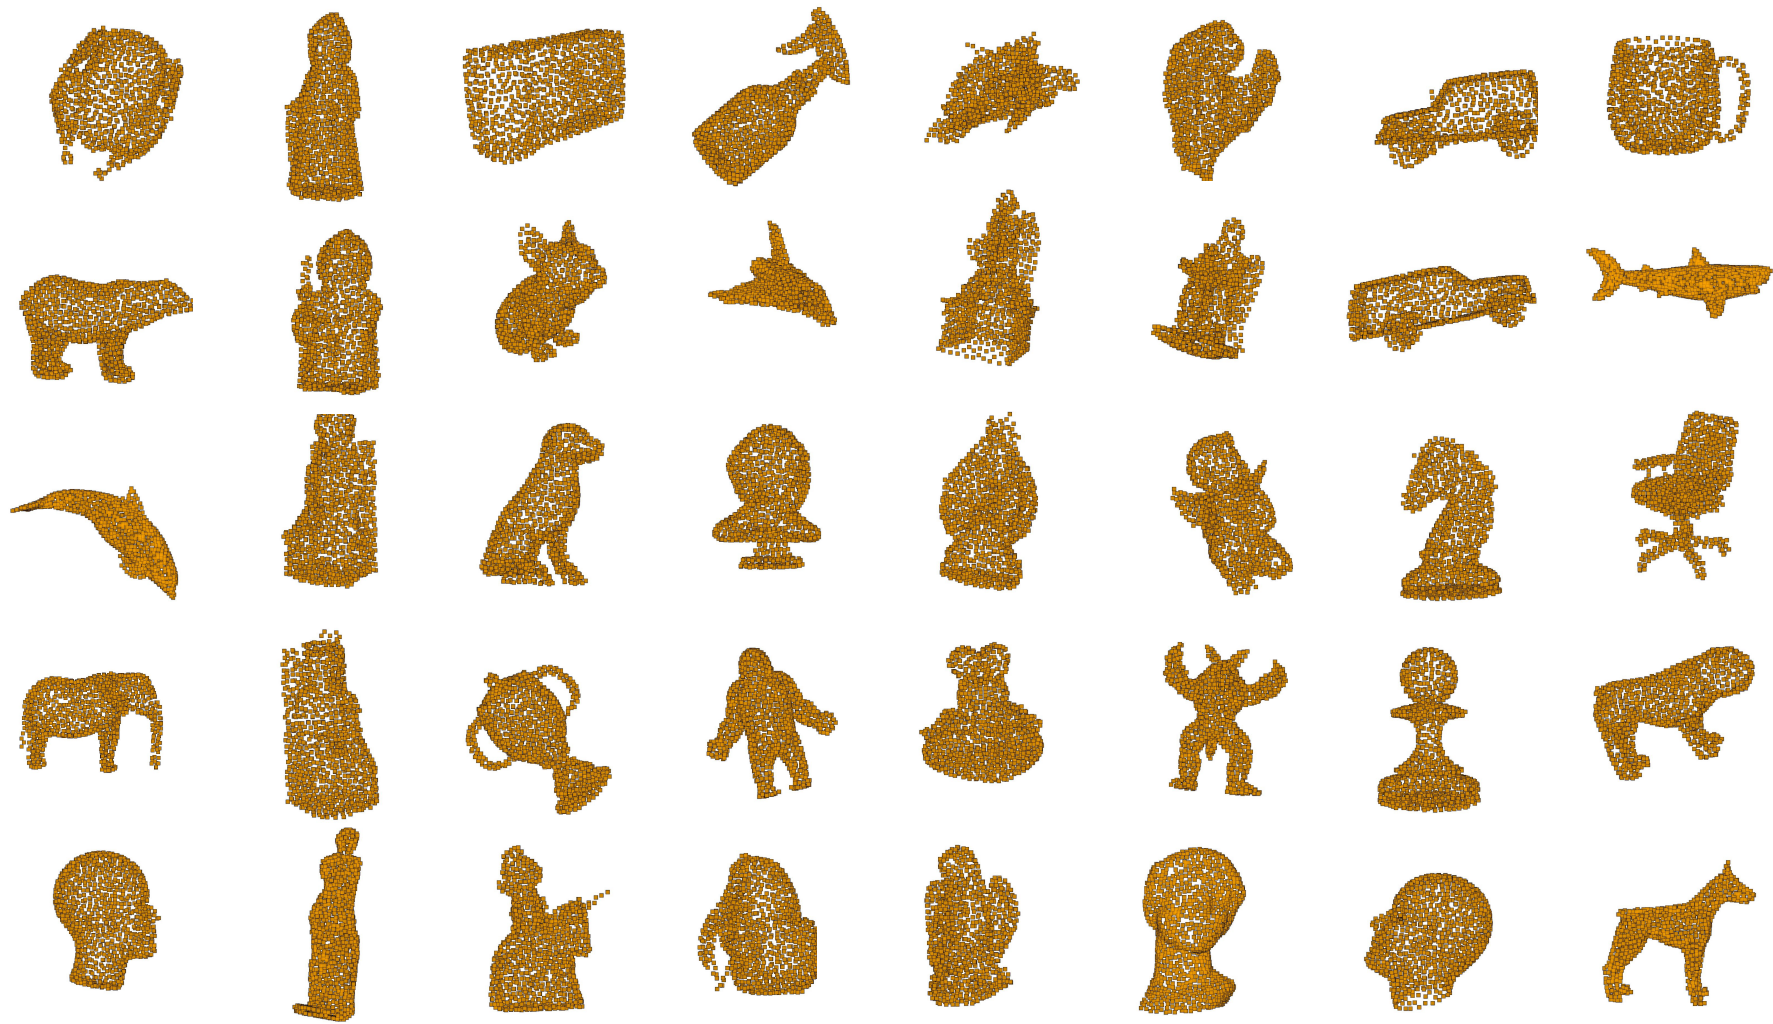

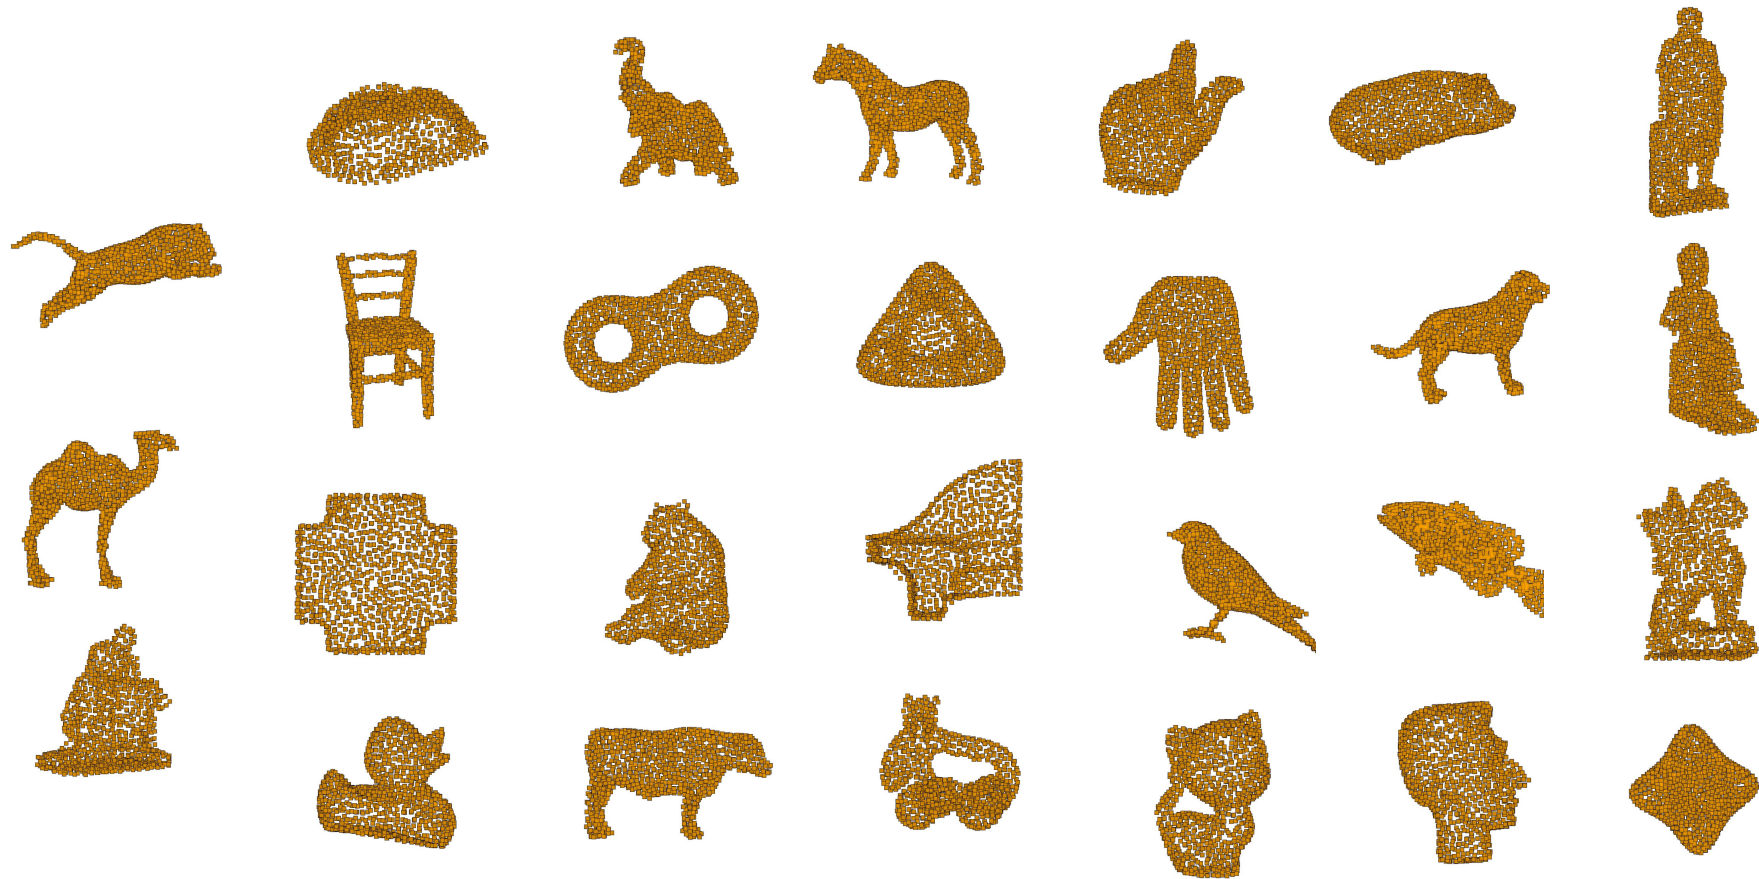

Supplement: Supplementary file 3 [file pugcn_cvpr21_supp.pdf]
